# Supplementary material for: Online Timestamp-based Transactional Isolation Checking of Database Systems (Extended Version)
Source: arXiv:2504.01477 source file (2025-04-02)
Supplement: Supplementary file 1 [file exp-si-violations.tex]

% exp-si-violations.tex

%%%%%%%%%%%%%%%%%%%%%%%%%%%%%%
\subsection{Finding SI Violations}
\label{ss:si-violations}
%%%%%%%%%%%%%%%%%%%%
\subsubsection{Reproducing Known SI Violations}
\label{sss:reproducing-si-violations}

% si-violations-known.tex

\begin{table}[t]
	\centering
	\caption{Known SI violations reproduced by \tool.}
	\label{table:si-violations-known}
  
  \resizebox{0.85\columnwidth}{!}{%
		\begin{tabular}{|c|c|c|}
			\hline
			{\bf Database} & {\bf Release} & {\bf Known SI Violations} \\ \hline\hline
			MongoDB & & \\ \hline
			TiDB & & \\ \hline
			YugabyteDB & & \\ \hline
			Dgraph & &  \\  \hline
		\end{tabular}
	}
\end{table}

We have successfully reproduced a variety of known SI violations
in the earlier releases of the four databases;
see Table~\ref{table:si-violations-known}.
%%%%%%%%%%%%%%%%%%%%
\subsubsection{Detecting New SI Violations}
\label{sss:detecting-si-violations}

% si-violations-new.tex

\begin{table}[t]
	\centering
	\caption{New SI violations found by \tool.}
	\label{table:si-violations-new}
  
  \resizebox{\columnwidth}{!}{%
		\begin{tabular}{|c|c|c|c|c|}
			\hline
			{\bf Database} & {\bf Release} & {\bf Known SI Violations} & {\bf Bug Report} & {\bf Status}
			\\ \hline\hline
			MongoDB & & & & \\ \hline
			TiDB & & & & \\ \hline
			YugabyteDB & & & & \\ \hline
			Dgraph & & & & \\ \hline
		\end{tabular}
	}
\end{table}

We use \tool{} to examine recent releases of these four databases.
and find \red{xxx} new SI violations in them.
We have reported these bugs to the developers \red{and}.
%\red{where xxx has been confirmed by the developers;
% xxx are investigating the issue.}
%%%%%%%%%%%%%%%%%%%%%%%%%
%%%%%%%%%%%%%%%%%%%%%%%%%%%%%%
