# Supplementary material for: Online Timestamp-based Transactional Isolation Checking of Database Systems (Extended Version)
Source: arXiv:2504.01477 source file (2025-04-02)
Supplement: Supplementary file 2 [file discussions.tex]

% discussions.tex

%%%%%%%%%%%%%%%%%%%%%%%%%%%%%%
\section{Discussions and Limitations}
\label{section:discussions}

%%%%%%%%%%%%%%%%%%%%
% \input{figs/ts-vs-nots}

% \paragraph*{Completeness of Timestamp-based Checking}
% The timestamp-based checking approach offers
% an additional advantage over the traditional black-box approach
% in terms of \emph{completeness}.
% The latter might overlook SI violations in certain histories
% from the perspective of database developers.
% For instance, consider the scenario depicted in Figure~\ref{fig:ts-vs-nots},
% where transactions $T_{1}$, $T_{2}$, and $T_{3}$
% are committed sequentially.
% Database developers envisioning the database's
% timestamp-based operational semantics
% might expect an SI violation,
% as $T_{3}$ reads from a snapshot that excludes the effect of $T_{2}$.
% However, traditional black-box SI checkers accept this history as SI,
% falsely inferring an execution order,
% i.e., $T_{1}$, $T_{3}$, $T_{2}$, which did not occur.

\paragraph*{On Strict Serializability Checking}
% Our approach is also applicable to the SER checking problem.
% The insight is that databases that implement SER
% aim to ensure that transactions appear to be executed
% in the increasing order of their commit timestamps.
% Implementing the timestamp-based checking approach
% and designing efficient checking algorithms for SER
% are generally simpler compared to those for snapshot isolation.

A number of databases,
such as Google Spanner~\cite{Spanner:OSDI2012,Spanner:TOCS2013},
FoundationDB~\cite{FoundationDB:SIGMOD2021},
and FaunaDB~\cite{FaunaDB},
have implemented strict serializability~\cite{Adya:PhDThesis1999}.
Checking strict serializability in our approach
entails accessing the \emph{wall-clock}
start and commit timestamps of each transaction.
We will explore how to faithfully obtain these timestamps.
% and design efficient checking algorithms for strict serializability.
%%%%%%%%%%%%%%%%%%%%
% \paragraph*{Data Types and Queries}

% Our approach is general and adaptable regardless of
% the data types and query languages used to generate the histories.
% We anticipate that extending \tool{} and \onlinetool{}
% to accommodate more data types such as sets, queues, and JSON documents,
% along with intricate queries like SQL range queries,
% SQL Join operator, and graph path queries,
% will be more feasible compared to other black-box checkers.
% We will explore this promising direction in our future work.
% This avenue will be explored in our future work.
%%%%%%%%%%%%%%%%%%%%
\paragraph*{Limitations}

To our knowledge, centralized databases like
SQL Server~\cite{SQLServer},
PostgreSQL~\cite{PostgreSQL}, and
WiredTiger~\cite{WiredTiger-Transaction}
implement SI in a similar manner,
without relying on timestamp-based mechanisms.
They associate each transaction with a unique identifier,
but the transaction identifiers, such as those used in WiredTiger,
may not directly correlate with the timestamps
employed in the database systems considered in this paper.
For instance, transactions are not necessarily
committed in the order of their identifiers.
Moreover, conditions like $T_{1}.\tid < T_{2}.\tid$
and $T_{2}$ being visible to $T_{3}$
do not necessarily imply that $T_{1}$ is also visible to $T_{3}$.
Thus, they utilize a {\it visibility rule} to
compute the snapshot of a transaction,
i.e., the \emph{set} of transaction identifiers visible to it.
We plan to extend our approach to handle such databases,
and further, to formally specify and verify these SI implementations.
%%%%%%%%%%%%%%%%%%%%
%%%%%%%%%%%%%%%%%%%%%%%%%%%%%%
