# Supplementary material for: Online Timestamp-based Transactional Isolation Checking of Database Systems (Extended Version)
Source: arXiv:2504.01477 source file (2025-04-02)
Supplement: Supplementary file 3 [file si-axiomatic.tex]

% si-axiomatic.tex

\begin{figure}[t]
	\centering
	\includegraphics[width = 0.40\textwidth]{figs/si-axiomatic}
	\caption{Illustration of the axiomatic semantics of SI.
	  (The arrows for $\ar$ implied by $\vis$ and transitivity are not shown.)}
	\label{fig:si-axiomatic}
\end{figure}
