# Supplementary material for: Online Timestamp-based Transactional Isolation Checking of Database Systems (Extended Version)
Source: arXiv:2504.01477 source file (2025-04-02)
Supplement: Supplementary file 4 [file si-op.tex]

% si-op.tex

\begin{figure}[t]
	\centering
	\includegraphics[width = 0.35\textwidth]{figs/si-op}
	\caption{Illustration of the operational semantics of SI.
	  The start and commit timestamps of each transaction
		are represented by dashed lines and dotted lines, respectively.
		All timestamps are totally ordered from left to right.}
	\label{fig:si-op}
\end{figure}
