# Supplementary material for: Online Timestamp-based Transactional Isolation Checking of Database Systems (Extended Version)
Source: arXiv:2504.01477 source file (2025-04-02)
Supplement: Supplementary file 5 [file si-checking-paper-454.pdf]

# CHRONOS and AION: Offline and Online Timestamp-based Checking of Snapshot Isolation in Database Systems

Anonymous Author(s)

## ABSTRACT

The snapshot isolation (SI) checking problem, which determines whether a given database execution satisfies SI, is fundamental to database testing. Most existing SI checkers treat the database system as a black-box, lacking insight into the underlying SI implementation and particularly the actual execution order of transactions. Consequently, these tools often face computational complexity issues and may be restricted to specific data types in database executions. Moreover, they are offline checkers with limited scalability.

To overcome these drawbacks, we propose a novel *timestamp-based* approach to SI checking. This approach requires database executions to include the start and commit timestamps of each transaction, making it applicable regardless of the data types used. By leveraging these timestamps, we can infer the actual execution order of transactions and determine the snapshot of each transaction. We have developed both offline and online highly efficient SI checking algorithms, named CHRONOS and AION, respectively. Experimental results demonstrate that CHRONOS can handle offline histories containing up to a million of transactions within tens of seconds, while existing black-box SI checkers take several hours or cannot handle such large histories at all. Moreover, AION can handle online transactional workloads with a sustained throughput of up to 3K transactions per second.

## KEYWORDS

transactional database system, isolation level, snapshot isolation, timestamps, black-box testing

### ACM Reference Format:

Anonymous Author(s). 2025. CHRONOS and AION: Offline and Online Timestamp-based Checking of Snapshot Isolation in Database Systems. In *Proceedings of the 2025 International Conference on Management of Data (SIGMOD '25)*. ACM, New York, NY, USA, 13 pages. <https://doi.org/XXXXXXX.XXXXXXX>

## 1 INTRODUCTION

Database transactions provide an “all-or-none” abstraction and isolate concurrent computations on shared data from each other [8], greatly simplifying client programming. The gold standard for transaction isolation is *serializability* (SER) [8, 23], which ensures that all transactions appear to execute serially, one after another. Unfortunately, ensuring SER is inevitably expensive [5]. Therefore, many databases choose to implement weaker isolation levels.

Permission to make digital or hard copies of all or part of this work for personal or classroom use is granted without fee provided that copies are not made or distributed for profit or commercial advantage and that copies bear this notice and the full citation on the first page. Copyrights for components of this work owned by others than the author(s) must be honored. Abstracting with credit is permitted. To copy otherwise, or republish, to post on servers or to redistribute to lists, requires prior specific permission and/or a fee. Request permissions from [permissions@acm.org](mailto:permissions@acm.org).  
SIGMOD '25, June 22–27, 2025, Berlin, Germany

© 2025 Copyright held by the owner/author(s). Publication rights licensed to ACM.  
ACM ISBN 978-1-4503-XXXX-X/18/06  
<https://doi.org/XXXXXXX.XXXXXXX>

Snapshot isolation (SI) [7] is one of the most popular weak isolation levels, implemented by both classic centralized databases like SQL Server [26], PostgreSQL [25], and WiredTiger [3] and emerging distributed databases like Google’s Percolator [24], MongoDB [22], TiDB [32], YugabyteDB [33], Dgraph [17], Memgraph [21], and Apache Omid [27]. However, it is notoriously difficult to implement databases correctly, with many databases failing to provide SI as they claim [20, 30, 31].

The SI checking problem asks whether a given database (execution) history satisfies SI, which is the basis of database testing. Researchers have designed several *black-box* checkers of SI, including dbcop [9], Elle [20], PolySI [19], and Viper [34]. In black-box settings, a history typically consists of a set of transactions issued by clients (also called sessions) to database, and typically records the transactions’ identifiers, the keys they read from or write to, and the corresponding values. In particular, it lacks the information of the actual execution order of these transactions.

There are several drawbacks associated with existing black-box SI checkers, i.e., dbcop, Elle, PolySI, and Viper:

- They are typically of *high complexity*. The SI checking problem has been proven to be NP-complete [9], even for histories with the *unique-value* (*UniqueValue*) assumption [9, 12, 19, 34] which requires that each key is written with unique values. In practice, dbcop, PolySI, and Viper use some domain-specific heuristics to prune the search space of possible execution orders of transactions in a history. However, they do not scale well to large histories with, e.g., tens of thousands of transactions, due to their exponential complexity in the worst case.
- They are not *general* enough for checking realistic histories generated in production. First, dbcop, PolySI, and Viper are limited to key-value stores. Although Elle can infer the execution order of transactions and check SI in polynomial time, it is restricted to databases that provide specific data types such as lists. Second, all of them rely on the *UniqueValue* assumption, which is not always satisfied in practice, and may miss the SI violations manifested only in histories without *UniqueValue*.
- All of them are *offline* checkers, which require the entire history to be available before checking. However, in practice, it is also desirable to check SI online, i.e., with continuous and ever-growing history. Cobra [29] supports online SER checking but not SI checking. Additionally, it needs to inject “fence transactions” into client workloads, which is often unacceptable in production.

*Our Approach.* To overcome the above drawbacks of existing black-box SI checkers, we propose the *timestamp-based* SI checking approach. This approach only requires a history also contains the start and commit timestamps of each transaction. The key insight of this approach is that, from commit timestamps, we can infer

the actual execution order of transactions; from start timestamps and the inferred execution order, we can determine the snapshot of each transaction. By simulating the execution of the transactions in the order of their commit timestamps and checking the rules of SI on the fly, we can design SI checkers (1) that are highly efficient, i.e., checking SI in polynomial time; (2) that are neither limited to specific data types nor to the UniqueValue assumption; and (3) that are suitable for online checking. See Section 3.1 for more insights.

The timestamp-based SI checking approach is practically feasible for two reasons.

- First, to our knowledge, most SI implementations in practice are timestamp-based (we discuss the exceptions in Section 6). Specifically, they all follow the high-level operational semantics of SI originally proposed by Berenson et al. [4, 7]. A transaction  $T$  reads versions of keys from a snapshot, which is associated with a *start-timestamp*, taken when it starts. The transaction commits only if it passes a write-write conflict detection check: since  $T$  started, no other committed transaction has written to any key that  $T$  also wrote to. If the check fails,  $T$  aborts. Once  $T$  commits, it is assigned a *commit-timestamp* and its changes become visible to all transactions that take a snapshot afterwards.
- Second, although transaction timestamps are typically not directly exposed to clients in database executions, they can be easily extracted from the responses to clients' transactional requests<sup>1</sup>, the logs, or the CDC (Change Data Capture) mechanism of the database systems. The timestamp-based SI checking can be as quite lightweight as the traditional black-box SI checking.

*Contributions.* Our approach is general and adaptable regardless of the data types used to generate the histories. In this work, we focus on SI checking for key-value histories and list histories (further discussions are presented in Section 6). Specifically, our contributions are as follows:<sup>2</sup>

- We propose a timestamp-based SI checking approach that addresses several drawbacks of existing black-box SI checkers and justify its feasibility in practice.
- (Section 3.2) We design a highly efficient offline timestamp-based SI checker named CHRONOS. It costs  $O(N \log N + M)$  time, where  $N$  and  $M$  are the number of transactions and operations in the history, respectively.
- (Section 3.3) We pose the challenges of online SI checking due to the inconsistency between the execution order and the checking order of transactions. To address these challenges, we extend CHRONOS to support online checking, which we call AION.
- (Sections 4 and 5) Finally, we evaluate both CHRONOS and AION under a wide range of workloads. Experimental results demonstrate that CHRONOS can handle offline histories containing up to a million of transactions within tens of seconds, while existing black-box SI checkers take several

<sup>1</sup>The *start* timestamps of each transaction are included in the HTTP responses of Dgraph. We have modified the source code of Dgraph to also include the *commit* timestamps in the HTTP responses, which has been officially merged into the main branch of Dgraph (to keep anonymity, we do not cite the specific pull request here).

<sup>2</sup>We have implemented the CHRONOS checker and the AION checker in 2.5k lines of Java code. Our tool, along with additional experimental data, is available at [1].

---

#### Algorithm 1 Operational Semantics of Snapshot Isolation

---

log: the log of committed transactions

```

1: procedure START( $T$ )
2:    $T.start\_ts \leftarrow \text{REQUEST}(O)$ 
3:   return ok
4: procedure WRITE( $T, k, v$ )
5:    $T.buffer \leftarrow T.buffer \circ \langle k, v \rangle$        $\triangleright$  append  $\langle k, v \rangle$  to  $T.buffer$ 
6:   return ok
7: procedure READ( $T, k$ )
8:   return value of  $k$  from  $T.buffer$  and log as of  $T.start\_ts$ 
9: procedure COMMIT( $T$ )
10:   $T.commit\_ts \leftarrow \text{REQUEST}(O)$ 
11:  if  $T$  conflicts with some concurrent transaction
12:    return aborted
13:   $\log \leftarrow \log \circ \langle T.buffer, T.commit\_ts \rangle$        $\triangleright$  append  $T$  to log
14:  return committed

```

---

hours or cannot handle such large histories at all. Moreover, AION can handle online transactional workloads with a sustained throughput of up to 3K transactions per second, with only a minor impact (approximately 5%) on the database throughput, attributed to history collection.

## 2 SEMANTICS OF SNAPSHOT ISOLATION

In this section, we review both the operational and axiomatic semantics of SI. In Section 3, we design our timestamp-based SI checking algorithms by relating these two semantics.

We consider a key-value store managing a set  $K$  of keys associated with values from  $V$ .<sup>3</sup> We use  $R(k, v)$  to denote a read operation that reads  $v \in V$  from  $k \in K$  and  $W(k, v)$  to denote a write operation that writes  $v \in V$  to  $k \in K$ .

### 2.1 SI: Operational Semantics

SI was first defined in [7]. The original definition is operational: it is describing how an implementation would work. We specify SI by showing a high-level implementation of it in Algorithm 1 [4, 28]. Each procedure in Algorithm 1 is executed atomically. We assume a time oracle  $O$  which returns a unique timestamp upon request and that the timestamps are totally ordered. In the paper, we reference pseudocode lines using the format “algorithm#:line#”.

When a transaction  $T$  starts, it is assigned a start timestamp  $T.start\_ts$  (line 1:2). The writes of  $T$  are buffered in  $T.buffer$  (line 1:5). Under SI, the transaction  $T$  reads data from its own write buffer and the snapshot (stored in log) of *committed* transactions valid as of its start time  $T.start\_ts$  (line 1:8). When  $T$  is ready to commit, it is assigned a commit timestamp  $T.commit\_ts$  (line 1:10) and allowed to commit if no other *concurrent* transaction  $T'$  (i.e.,  $[T'.start\_ts, T'.commit\_ts]$  and  $[T.start\_ts, T.commit\_ts]$  overlap) has already written data that  $T$  intends to write (line 1:11). This rule prevents the “lost updates” anomaly. If  $T$  commits, it appends its buffered writes, along with its commit timestamp, to log (line 1:13).

<sup>3</sup>We assume an artificial value  $\perp_v \notin V$ .

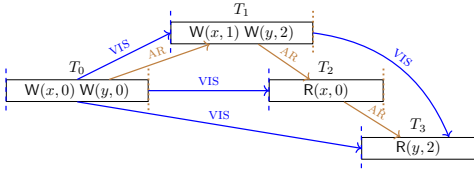

**Figure 1: Illustration of both the operational and axiomatic semantics of SI. The start and commit timestamps are represented by dashed lines and dotted lines, respectively. All timestamps are totally ordered from left to right. (The arrows for AR implied by VIS and transitivity are not shown.)**

The start and commit timestamps of a transaction  $T$  can be wall time or logical time. We require that for each transaction  $T$ ,

$$T.start\_ts \leq T.commit\_ts. \quad (1)$$

Note that we allow  $T.commit\_ts = T.start\_ts$ , which is possible for read-only transactions.

*Example 2.1.* Figure 1 shows a valid execution history of SI according to Algorithm 1 (ignore the edges for now). In this history, the snapshot taken by  $T_2$  does not contain the effect of  $T_1$ , since  $T_1.commit\_ts > T_2.start\_ts$ . In contrast, the snapshot taken by  $T_3$  contains the effect of  $T_1$ , thereby reading 2 from  $y$  written by  $T_1$ .

## 2.2 SI: Axiomatic Semantics

To define the axiomatic semantics of SI, we first introduce the formal definitions of transactions, histories, and abstract executions [11].

In this paper, we use  $(a, b) \in R$  and  $a \xrightarrow{R} b$  interchangeably, where  $R \subseteq A \times A$  is a relation over the set  $A$ . We write  $\text{Dom}(R)$  for the domain of  $R$ . Given two relations  $R$  and  $S$ , their composition is defined as  $R ; S = \{(a, c) \mid \exists b \in A : a \xrightarrow{R} b \xrightarrow{S} c\}$ . A strict partial order is an irreflexive and transitive relation. A strict total order is a relation that is a strict partial order and total.

*Definition 2.2.* A transaction is a pair  $(O, po)$ , where  $O$  is a set of operations and  $po \subseteq O \times O$  is the program order over  $O$ .

Clients interact with the store by issuing transactions during sessions. We use a history to record the client-visible results of such interactions.

*Definition 2.3.* A history is a pair  $\mathcal{H} = (\mathcal{T}, SO)$ , where  $\mathcal{T}$  is a set of transactions and  $SO \subseteq \mathcal{T} \times \mathcal{T}$  is the session order over  $\mathcal{T}$ .

We assume that every history contains a special transaction  $\perp_T$  that writes the initial values of all keys [9, 10, 12]. This transaction precedes all the other transactions in  $SO$ .

To declaratively justify each transaction of a history, we need to establish the visibility and arbitration relations among transactions. The visibility relation specifies the set of transactions whose effects are visible to each transaction, while the arbitration relation specifies the execution order of transactions.

*Definition 2.4.* An abstract execution is a tuple  $\mathcal{A} = (\mathcal{T}, SO, VIS, AR)$ , where  $(\mathcal{T}, SO)$  is a history, visibility  $VIS \subseteq \mathcal{T} \times \mathcal{T}$  is a strict partial order, and arbitration  $AR \subseteq \mathcal{T} \times \mathcal{T}$  is a strict total order such that  $VIS \subseteq AR$ .

*Definition 2.5 (Snapshot Isolation (Axiomatic) [11, 12]).* A history  $\mathcal{H} = (T, SO)$  satisfies SI if and only if there exists an abstract execution  $\mathcal{A} = (T, SO, VIS, AR)$  such that the SESSION, INT, EXT, PREFIX, and NoCONFLICT axioms (explained below) hold.

Let  $r \triangleq R(k, \_)$  be a read operation of transaction  $T$ . If  $r$  is the first operation on  $k$  in  $T$ , then it is called an *external* read operation of  $T$ ; otherwise, it is an *internal* read operation.

The *internal consistency axiom* INT ensures that, within a transaction, an internal read from a key returns the same value as the last write to or read from this key in the transaction. The *external consistency axiom* EXT ensures that an external read in a transaction  $T$  from a key returns the final value written by the last transaction in AR among all the transactions that precede  $T$  in terms of VIS and write to this key.

The SESSION axiom (i.e.,  $SO \subseteq VIS$ ), requires previous transactions be visible to transactions later in the same session.<sup>4</sup> The PREFIX axiom (i.e.,  $AR ; VIS \subseteq VIS$ ) ensures that if the snapshot taken by a transaction  $T$  includes a transaction  $S$ , then this snapshot also include all transactions that committed before  $S$  in terms of AR. The NoCONFLICT axiom prevents concurrent transactions from writing on the same key. That is, for any conflicting transactions  $S$  and  $T$ , one of  $S \xrightarrow{VIS} T$  and  $T \xrightarrow{VIS} S$  must hold.

*Example 2.6.* Figure 1 shows that the history is also valid under the axiomatic semantic of SI. It constructs a possible abstract execution by establishing the visibility and arbitration relations as shown in the figure. For example,  $T_0$  is visible to  $T_2$  but  $T_1$  is not. Both  $T_0$  and  $T_1$  are visible to  $T_3$ . Since  $T_1$  is after  $T_0$  in terms of AR,  $T_3$  reads the value 2 of  $y$  written by  $T_1$ .

## 3 TIMESTAMP-BASED SI CHECKING ALGORITHMS

We first describe the insights behind our timestamp-based SI checking algorithms and explain how they overcome the drawbacks of existing SI checkers mentioned in Section 1.

### 3.1 Insights

Consider a database history  $\mathcal{H} = (\mathcal{T}, SO)$  generated by Algorithm 1. We need to check whether  $\mathcal{H}$  satisfies SI by constructing an abstract execution  $\mathcal{A} = (\mathcal{T}, SO, VIS, AR)$  with appropriate relations VIS and AR on  $\mathcal{T}$ . The key insight of our approach is to infer the actual execution order of transactions to be consistent with their commit timestamps. Formally, we define AR as follows.

*Definition 3.1 (Timestamp-based Arbitration).*

$$\forall T_1, T_2 \in \mathcal{T}. T_1 \xrightarrow{AR} T_2 \iff T_1.commit\_ts < T_2.commit\_ts. \quad (2)$$

On the other hand, from start timestamps and the inferred execution order, we can determine the snapshot of each transaction: each transaction observes the effects of all transactions that have committed before it starts. Formally, we define VIS as follows.

*Definition 3.2 (Timestamp-based Visibility).*

$$\forall T_1, T_2 \in \mathcal{T}. T_1 \xrightarrow{VIS} T_2 \iff T_1.commit\_ts \leq T_2.start\_ts. \quad (3)$$

<sup>4</sup>That is, we consider the *strong session* variant of SI [12, 16] commonly used in practice.

*Example 3.3.* The VIS and AR relations of Figure 1 are constructed according to Definitions 3.2 and 3.1, respectively. For example, four transactions in the history are totally ordered (in AR) by their commit timestamps. On the other hand, since  $T_1.commit\_ts < T_3.start\_ts$ , we have  $T_1 \xrightarrow{VIS} T_3$ .

Given the VIS and AR relations, it is straightforward to show that the PREFIX axiom holds, i.e.,  $AR \vdash VIS \subseteq VIS$ . Therefore, by Definition 2.5, it remains to check that the SESSION, INT, EXT, and NOCONFLICT axioms hold. Since transactions are totally ordered, our checking algorithms can *simulate* transaction execution one by one, following their commit timestamps, and check the axioms on the fly. This simulation approach enables highly efficient checking algorithms that eliminate the need to explore all potential transaction execution orders within a history, as required by PolySI [19] and Viper [34], or to conduct expensive cycle detection on extensive dependency graphs of histories, as required by Elle [20]. Moreover, this simulation is not restricted to specific data types or the Unique-Value assumption, as long as the sequential semantics of the data type is provided. Lastly, the incremental nature of the simulation renders our algorithms suitable for online checking.

## 3.2 The CHRONOS Offline Checking Algorithm

**3.2.1 Input.** CHRONOS takes a history  $\mathcal{H}$  as input and checks whether it satisfies SI. Each transaction  $T$  in the history is associated with the following data:

- $T.tid$ : the unique ID of  $T$ . We use TID to denote the set of all transaction IDs in  $\mathcal{H}$ ;
- $T.sid$ : the unique ID of the session to which  $T$  belongs. We use SID to denote the set of all session IDs in  $\mathcal{H}$ ;
- $T.sno$ : the sequence number of  $T$  in its session;
- $T.ops$ : the list of operations in  $T$ ; and
- $T.start\_ts, T.commit\_ts$ : the start and commit timestamp of  $T$ , respectively. We use TS to denote the set of all timestamps in  $\mathcal{H}$  and denote the minimum timestamp in TS by  $\perp_{ts}$ .

We use  $T.wkey$  to record the set of keys written by  $T$ . We design CHRONOS with key-value histories in mind, but it is also easily adaptable to support other data types such as lists.

**3.2.2 Algorithm.** CHRONOS simulates the execution of a database assuming that the start and commit events of transactions in  $\mathcal{H}$  are executed in the order of their timestamps, while checking the corresponding axioms on the fly. To do this, CHRONOS sorts all the timestamps in TS in ascending order (line 2:2). By Definition 3.1, we obtain the total order AR between transactions. CHRONOS will traverse TS in this order and process each of the start events and commit events of transactions one by one (line 2:3). During this process, CHRONOS maintains two maps: *frontier* maps each key to the last (in AR) committed value, and *ongoing* maps each key to the set of ongoing transactions that write this key.

Let  $ts$  be the current timestamp being processed and  $T$  the transaction that owns the timestamp  $ts$ . If  $ts$  is the start timestamp of  $T$ , CHRONOS checks whether  $T$  violates any of the SESSION, INT, and EXT axioms (line 2:6). Otherwise, it checks whether  $T$  violates the NOCONFLICT axiom (line 2:23). CHRONOS will identify *all* violations of these axioms in a history, instead of terminating immediately upon encountering the first one.

### Algorithm 2 CHRONOS: the offline SI checking algorithm

---

```

last_sno  $\in$  SID  $\rightarrow \mathbb{N}$ :  $sno$  of the last transaction already processed
in each session, initially  $-1$ 
last_cts  $\in$  SID  $\rightarrow$  TS:  $commit\_ts$  of the last transaction already
processed in each session, initially  $\perp_{ts}$ 
frontier  $\in$  K  $\rightarrow$  V: the last committed value of each key, initially  $\perp_v$ 
ongoing  $\in$  K  $\rightarrow 2^{TID}$ : the set of ongoing transactions on each key,
initially  $\emptyset$ 
int_val  $\in$  TID  $\rightarrow$  (K  $\rightarrow$  V): the last read/written value of each key
in each transaction, initially  $\perp_v$ 
ext_val  $\in$  TID  $\rightarrow$  (K  $\rightarrow$  V): the last written value of each key
in each transaction, initially  $\perp_v$ 

1: procedure CHECKSI( $\mathcal{H}$ )  $\triangleright \mathcal{H}$  contains the initial transaction  $\perp_T$ 
2:   sort TS in ascending order
3:   for  $ts \in$  TS
4:      $T \leftarrow$  the transaction that owns the timestamp  $ts$ 
5:      $sid \leftarrow T.sid$     $tid \leftarrow T.tid$     $T.wkey \leftarrow \emptyset$ 
6:     if  $ts = T.start\_ts$   $\triangleright$  start event of  $T$ 
7:       if  $T.sno \neq last\_sno[sid] + 1 \vee T.start\_ts < last\_cts[sid]$ 
8:         report a violation of SESSION
9:        $last\_sno[sid] \leftarrow T.sno$ 
10:       $last\_cts[sid] \leftarrow T.commit\_ts$ 
11:      for ( $op = \_ (k, v)$ )  $\in T.ops$   $\triangleright$  in program order
12:        if  $op = R(k, v)$ 
13:          if  $int\_val[tid][k] = \perp_v$   $\triangleright$  external read
14:            if  $v \neq frontier[k]$ 
15:              report a violation of EXT
16:          else if  $int\_val[tid][k] \neq v$   $\triangleright$  internal read
17:            report a violation of INT
18:          else  $\triangleright op = W(k, v)$ 
19:             $T.wkey \leftarrow T.wkey \cup \{k\}$ 
20:             $ext\_val[tid][k] \leftarrow v$ 
21:             $ongoing[k] \leftarrow ongoing[k] \cup \{tid\}$ 
22:             $int\_val[tid][k] \leftarrow v$ 
23:          else  $\triangleright$  commit event of  $T$ 
24:            if  $T.start\_ts > T.commit\_ts$   $\triangleright$  check Eq. (1)
25:              report an error
26:            for  $k \in T.wkey$ 
27:               $ongoing[k] \leftarrow ongoing[k] \setminus \{tid\}$   $\triangleright$  except  $T$  itself
28:              if  $ongoing[k] \neq \emptyset$ 
29:                report a violation of NOCONFLICT
30:               $frontier[k] \leftarrow ext\_val[tid][k]$ 
31:               $int\_val[tid] \leftarrow \emptyset$   $\triangleright$  gc int_val
32:               $ext\_val[tid] \leftarrow \emptyset$   $\triangleright$  gc ext_val
33:               $\mathcal{T} \leftarrow \mathcal{T} \setminus \{T\}$   $\triangleright$  gc  $T$ 

```

---

**SESSION (lines 2:7 – 2:10).** CHRONOS uses  $last\_sno$  and  $last\_cts$  to maintain the  $sno$  and  $commit\_ts$  of the last transaction already processed in each session, respectively. It checks whether the current transaction  $T$  follows immediately after the last transaction already processed in its session and starts after this last transaction commits. If this fails, a violation of SESSION is found.

**INT and EXT (lines 2:12 – 2:17).** Let  $tid \triangleq T.tid$ . CHRONOS uses  $int\_val[tid][k]$  to track the last value read or written by  $T$  on key

$k$  (see line 2:22). Let  $op = R(k, v)$  be the read operation of  $T$  being checked (line 2:12). If  $\text{int\_val}[tid][k]$  is not the initial artificial value  $\perp_v$ , then  $op$  is an internal read. CHRONOS then checks if  $\text{int\_val}[tid][k] = v$ . If this fails, a violation of INT is found (line 2:17).

If  $\text{int\_val}[tid][k] = \perp_v$ , then  $op$  is an external read (line 2:13). By EXT,  $op$  should observe the last committed value of  $k$ , i.e.,  $\text{frontier}[k]$ . Otherwise, a violation of EXT is found (line 2:15).

For a key  $k$ , CHRONOS updates  $\text{frontier}[k]$  whenever a transaction that writes to  $k$  commits. Since a transaction  $T$  may write to the same key  $k$  multiple times, CHRONOS uses  $\text{ext\_val}[tid][k]$  to track the last value written by  $T$  on  $k$  (see line 2:20). Therefore, when  $T$  commits, CHRONOS updates  $\text{frontier}[k]$  to  $\text{ext\_val}[tid][k]$  (line 2:30).

**NoCONFLICT** (lines 2:27 – 2:29). Now suppose that  $ts$  is the commit timestamp of  $T$  (line 2:23). For each key  $k \in T.\text{wkey}$  written by  $T$  (tracked at line 2:19), CHRONOS checks whether  $T$  conflicts with any ongoing transactions on key  $k$  by testing the emptiness of  $\text{ongoing}[k]$  (tracked at line 2:21). If  $\text{ongoing}[k]$  (except  $T$  itself) is non-empty, a violation of NoCONFLICT is found (line 2:29).

**GARBAGECOLLECT** (lines 2:30 – 2:33). To save memory, CHRONOS periodically discard obsolete information from  $\text{int\_val}$  and  $\text{ext\_val}$  and remove old transactions from  $\mathcal{T}$ . First, it is safe to discard  $\text{int\_val}[tid]$  once the commit event of transaction  $T$  has been processed (line 2:31), since the information in  $\text{int\_val}$  will never be used by any other transaction. Second, for a transaction  $T$ , all of its writes have been recorded in  $\text{frontier}$ ,  $\text{ext\_val}[tid]$  becomes redundant and can be discarded (line 2:32). Furthermore,  $T.\text{sno}$  and  $T.\text{cts}$  are recorded in  $\text{last\_sno}$  and  $\text{last\_cts}$ , respectively, and thus  $T$  is no longer needed in  $\mathcal{T}$  (line 2:33).

*Example 3.4.* Consider the history of Figure 2 which consists of five transactions, namely  $T_1, T_2, \dots$ , and  $T_5$ . CHRONOS processes the start and commit events of the transactions in the ascending order of their timestamps, namely ❶, ❷,  $\dots$ , and ❿.

On the start event of  $T_3$  with timestamp ❸, the external read operation  $R(x, 2)$  can be justified by the last committed transaction  $T_2$  that writes 2 to  $x$ . This is captured by the current  $\text{frontier}[x] = \{T_2\}$ . Moreover, since  $T_3$  updates key  $y$ , CHRONOS adds  $T_3$  to  $\text{ongoing}[y]$ , yielding  $\text{ongoing}[y] = \{T_3\}$ . Now comes the commit event of  $T_5$  with timestamp ❶. CHRONOS finds that  $T_5$  conflicts with  $T_3$  on  $y$  by checking the emptiness of  $\text{ongoing}[y] \setminus \{T_5\}$ , reporting a violation of NoCONFLICT. In addition, since  $T_5$  updates key  $y$ , CHRONOS updates  $\text{frontier}[y]$  to  $\{T_5\}$ . This justifies the external read operation  $R(y, 1)$  of  $T_4$  when CHRONOS examines the start event of  $T_4$  with timestamp ❹. Note that upon the commit event of  $T_3$  with timestamp ❷, CHRONOS does *not* report a violation of NoCONFLICT for  $T_3$  with  $T_5$  on  $y$  because this violation has already been reported on the commit event of  $T_5$  and now  $T_5 \notin \text{ongoing}[y]$  at line 2:27.

**3.2.3 Complexity Analysis.** Suppose that the history  $\mathcal{H}$  consists of  $N$  transactions and  $M$  operations ( $N \leq M$ ). We assume that the data structures used by CHRONOS are implemented as hash maps (or hash sets) which offer average constant time performance for the basic operations like put, get, remove, contains, and isEmpty.

The time complexity of CHRONOS comprises

- $O(N \log N)$  for sorting on TS (line 2:2);

- $O(N) = N \cdot O(1)$  for checking SESSION on the start events of transactions (lines 2:7 – 2:10);
- $O(M) = M \cdot O(1)$  for checking EXT and INT on each read operation of transactions (lines 2:12 – 2:17) and for updating data structures on each write operation of transactions (lines 2:18 – 2:21);
- $O(N) = N \cdot O(1)$  for checking Eq. (1) on the commit events of transactions (lines 2:24 – 2:25);
- $O(M) = O(M) \cdot O(1)$  for checking NoCONFLICT on the commit events of transactions (lines 2:27 – 2:29).

Therefore, the time complexity of CHRONOS is  $O(N \log N + M)$ .

The space complexity of CHRONOS is primarily determined by the memory required for storing the history (the memory usage of the frontier and ongoing data structures is relatively small). Thanks to its prompt garbage collection mechanism, the memory usage for storing the history diminishes as transactions are processed.

### 3.3 The AION Online Checking Algorithm

**3.3.1 Input.** In the online settings, the history  $\mathcal{H}$  is not known in advance. Instead, the online checking algorithm AION receives transactions one by one and checks SI incrementally. It is assumed that the session order is preserved when transactions are received.

**3.3.2 Challenges.** Due to asynchrony, AION *cannot* anticipate that transactions will be collected in ascending order based on their start/commit timestamps. This introduces three main challenges for AION.

- The determination of satisfaction or violation of the EXT axiom for a transaction becomes *unstable* due to asynchrony. This means that we cannot assert it immediately upon the transaction being collected. In contrast, the INT axiom remains unaffected by asynchrony, while NoCONFLICT violations will eventually be correctly reported as soon as the conflicting transactions are collected.
- An incoming transaction  $T$  with a smaller start timestamp may initiate the *re-checking* of transactions that commit after  $T$  starts. To facilitate efficient rechecking, it is essential to extend and maintain the data structures, namely frontier and ongoing.
- To prevent unlimited memory usage and facilitate long-running checking, AION must recycle data structures and transactions that are no longer necessary. Unfortunately, in the worst-case scenario, AION cannot safely recycle any data structures and transactions due to asynchrony.

The following example illustrates the challenges faced by AION and our solutions to overcome them.

*Example 3.5.* Consider the history of Figure 2. Suppose that the five transactions are collected in the order  $T_1, T_2, \dots$ , and  $T_5$ .

When AION collects the first four transactions, it cannot definitively assert that  $T_4$  violates the EXT axiom permanently. This uncertainty arises because  $T_5$ , from which  $T_4$  reads the value of  $y$ , may experience delays due to asynchrony. To tackle this instability issue, AION employs a waiting period during which delayed transactions are expected to be collected. This approach allows for a more accurate determination of whether a violation of EXT persists or is a transient result of asynchrony.

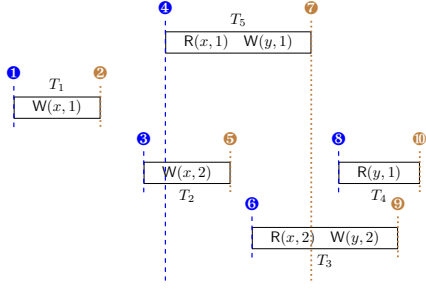

**Figure 2: Illustration of both the offline checking algorithm CHRONOS (in Example 3.4) and the online checking algorithm AION (in Example 3.5).**

Now, when transaction  $T_5$  arrives, AION must check the SESSION, INT, and EXT axioms for  $T_5$  and *re-check* all transactions that commit after  $T_5$  starts (denoted ④). The re-checking process involves two cases based on the axioms to be verified: (1) re-check the NoCONFLICT axiom for transactions overlapping with  $T_5$ , i.e.,  $T_2$  and  $T_3$  in this example; and (2) re-check the EXT axiom for transactions starting after  $T_5$  commits, i.e.,  $T_4$  in this example. To facilitate this, the data structures *frontier* and *ongoing* should be *versioned* by timestamps and support timestamp-based search, returning the latest version *before* a given timestamp.

For instance, to determine the set of transactions overlapping with  $T_5$  (for checking the NoCONFLICT axiom), AION queries the versioned data structure *ongoing* using the timestamp  $T_5.commit\_ts$  ⑦ (and key  $y$ ). This query returns the set of ongoing transactions updated at timestamp  $T_3.start\_ts$  ⑥, namely  $\{T_3.tid\}$ . Consequently, AION identifies a conflict between  $T_5$  and  $T_3$  and reports a violation of the NoCONFLICT axiom.

Similarly, to justify the read operation  $R(y, 1)$  of  $T_4$  (for re-checking the EXT axiom), AION queries the versioned data structure *frontier* using the timestamp  $T_4.start\_ts$  ⑧ (and key  $y$ ). This query returns the frontier updated at timestamp  $T_5.commit\_ts$  ⑦, namely  $[y \mapsto 1]$ . Thus,  $T_4$  is re-justified by  $T_5$ , clearing the false alarm on the violation of EXT axiom for  $T_5$ . Be cautious that this result is also temporary and subject to change due to asynchrony.

For violations of the INT, EXT, and NoCONFLICT axiom, AION reports the violation and continues checking as if the violation did not occur.

**3.3.3 Algorithm.** Algorithm 3 provides the pseudocode for AION. AION extends the data structures *frontier* and *ongoing* used in CHRONOS to *frontier\_ts* and *ongoing\_ts*, respectively, which are versioned by timestamps. When given a timestamp  $ts$ , we use  $frontier\_ts[ts]$  and  $ongoing\_ts[ts]$  to denote the latest version of *frontier\_ts* and *ongoing\_ts* *before*  $ts$ , respectively.

Upon receiving a new transaction  $T$ , AION proceeds in three steps: it first checks the SESSION, INT, and EXT axioms for  $T$ , similarly to CHRONOS (lines 3:6 – 3:25), then it re-checks the NoCONFLICT axiom for transactions overlapping with  $T$  (lines 3:26 – 3:35), and finally, it re-checks the EXT axiom for transactions starting after  $T$  commits (lines 3:37 – 3:57).

**Step ① (lines 3:6 – 3:25).** The checking for  $T$  is similar to that in CHRONOS, with two differences. On one hand, to check the EXT axiom, AION needs to obtain the latest version of *frontier\_ts* before  $T.start\_ts$ , denoted  $frontier\_ts[T.start\_ts]$  (line 3:14). Moreover, to update *frontier\_ts* at timestamp  $cts \leftarrow T.commit\_ts$ , it first fetches the latest version of *frontier\_ts* before  $cts$  (line 3:23) and then updates the components for each key written by  $T$  (line 3:24). On the other hand, if  $T$  violates the EXT axiom, AION does not report the violation immediately as it is subject to change due to asynchrony. Instead, it records the temporary violation in variable  $T.EXT$  (line 3:15) and waits for a timeout (line 3:59) set at the beginning (line 3:3).

**Step ② (lines 3:26 – 3:35).** To re-check the NoCONFLICT axiom for transactions overlapping with  $T$ , AION iterates through the timestamps  $ts$  ranging from  $T.start\_ts$  to  $T.commit\_ts$  (both *inclusive*) in ascending order (line 3:26). If  $ts$  corresponds to the start timestamp of a transaction  $T'$  (which could be  $T$ ), AION updates  $ongoing\_ts[ts]$  for each key written by  $T'$  (line 3:30) to include  $T'.tid$ . If  $ts$  corresponds to the commit timestamp of transaction  $T'$ , AION reports that  $T'$  conflicts with the set of ongoing transactions in  $ongoing\_ts[ts][k]$  for each key  $k$  written by  $T'$  (line 3:34). Note that we exclude  $T'.tid$  from  $ongoing\_ts[ts]$  at line 3:33 to prevent reporting self-conflicts (i.e.,  $T'$  conflicting with itself). This also prevents reporting duplicate conflicts: in the case of conflicting transactions  $T_1$  and  $T_2$ , AION reports the conflict only once, considering the transaction with the smaller commit timestamp.

**Step ③ (lines 3:37 – 3:57).** To re-check the EXT axiom for transactions starting after  $T$  commits, AION iterates through timestamps  $ts$  greater than  $T.commit\_ts$  in ascending order (line 3:37). If  $ts$  corresponds to the start timestamp of a transaction  $T'$  and the timeout for  $T'$  has not expired, AION re-checks the EXT axiom for each external read of  $T'$  based on  $ext\_val[T]$  (line 3:43), instead of using the latest version of *frontier\_ts* before  $ts$  as in *Step ①*. This optimization is effective because only the recently incoming transaction  $T$  impacts the justification of external reads of  $T'$ . For further optimization, AION re-checks only the external reads of  $T'$  on keys that are written by  $T$  (line 3:36 and line 3:43) and have not been overwritten by later transactions after  $T$  (line 3:53). Essentially, the values of these keys are still influenced by  $T$ . Therefore, if  $ts$  corresponds to the commit timestamp of transaction  $T'$ , it suffices for AION to update  $frontier\_ts[ts]$  only for these keys (line 3:57). The third optimization dictates that once all keys written by  $T$  are overwritten by later transactions, the re-checking process for EXT terminates (line 3:55).

The determination of violation or satisfaction of the EXT axiom at this stage is temporary and recorded in  $T'.EXT$  (line 3:45 and line 3:47). When the timeout for  $T'$  expires, AION reports an EXT violation if  $T'.EXT = \perp$  (line 3:61).

**GARBAGECOLLECT (lines 3:63 – 3:66).** As previously mentioned, in the worst-case scenario, AION cannot safely recycle any data structures or transactions due to asynchrony. To mitigate memory usage, AION performs garbage collection periodically and conservatively: each time it transfers *frontier\_ts*, *ongoing\_ts*, and transactions below a specified timestamp from memory to disk (lines 3:63 – 3:66, marked

---

**Algorithm 3** AION: the online SI checking algorithm

---

last\_sno, last\_cts, int\_val, and ext\_val are the same as in CHRONOS

```

1: procedure ONLINECHECKSI( $T$ )  $\triangleright$  upon receiving a new transaction  $T$ 
2:    $T.EXT \leftarrow \top$   $\triangleright T.EXT$ : whether  $T$  satisfies EXT, initially true
3:   set a timer for re-checking EXT for  $T$ 
4:   if  $T.start\_ts > T.commit\_ts$   $\triangleright$  check Eq. (1)
5:     report an error
6:    $sid \leftarrow T.sid$     $tid \leftarrow T.tid$     $T.wkey \leftarrow \emptyset$ 
    $\triangleright$  ① check SESSION, INT, and EXT for  $T$ , similarly to CHRONOS
7:   if  $T.sno \neq last\_sno[sid] + 1 \vee T.start\_ts < last\_cts[sid]$ 
8:     report a violation of SESSION
9:    $last\_sno[sid] \leftarrow T.sno$ 
10:   $last\_cts[sid] \leftarrow T.commit\_ts$ 
11:  for  $(op = \_ (k, v)) \in T.ops$ 
12:    if  $op = R(k, v)$ 
13:      if  $int\_val[tid][k] = \perp_v$   $\triangleright$  external read
14:        if  $v \neq frontier\_ts[\widehat{T.start\_ts}][k]$   $\uparrow$ 
15:           $T.EXT \leftarrow \perp$ 
16:        else if  $int\_val[tid][k] \neq v$   $\triangleright$  internal read
17:          report a violation of INT
18:        else  $\triangleright op = W(k, v)$ 
19:           $T.wkey \leftarrow T.wkey \cup \{k\}$ 
20:           $ext\_val[tid][k] \leftarrow v$ 
21:           $int\_val[tid][k] \leftarrow v$ 
22:         $cts \leftarrow T.commit\_ts$ 
23:         $frontier\_ts[cts] \leftarrow frontier\_ts[cts]$   $\uparrow$ 
24:         $frontier\_ts[cts][k] \leftarrow ext\_val[tid][k]$  for  $k \in T.wkey$ 
25:         $int\_val[tid][k] \leftarrow \perp_v$  for  $k \in Dom(int\_val[tid])$   $\triangleright$  reset
    $\triangleright$  ② re-check NoCONFLICT for transactions overlapping with  $T$ 
26:  for  $ts \in TS$  such that  $T.start\_ts \leq ts \leq T.commit\_ts$ 
27:     $T' \leftarrow$  the transaction that owns the timestamp  $ts$   $\uparrow$ 
28:    if  $ts = T'.start\_ts$ 
29:      for  $k \in T'.wkey$ 
30:         $ongoing\_ts[ts][k] \leftarrow ongoing\_ts[\widehat{ts}][k] \cup \{T'.tid\}$   $\uparrow$ 
31:      else  $\triangleright ts = T'.commit\_ts$ 
32:        for  $k \in T'.wkey$ 
33:           $ongoing\_ts[ts][k] \leftarrow ongoing\_ts[\widehat{ts}][k] \setminus \{T'.tid\}$   $\uparrow$ 
34:          if  $ongoing\_ts[ts][k] \neq \emptyset$ 
35:            report a violation of NoCONFLICT

36:   $frontier\_ts \in TS \rightarrow (K \rightarrow V)$  : frontier versioned by timestamps
37:   $ongoing\_ts \in TS \rightarrow (K \rightarrow 2^{TID})$  : ongoing versioned by timestamps
    $\triangleright$  ③ re-check EXT for transactions starting after  $T$  commits
38:   $keys \leftarrow T.wkey$ 
39:  for  $ts \in TS$  such that  $ts > T.commit\_ts$ 
40:     $T' \leftarrow$  the transaction that owns the timestamp  $ts$   $\uparrow$ 
41:    if  $ts = T'.start\_ts$ 
42:      if TIMEOUT( $T'$ ) has been called
43:        continue
44:      for  $(op = \_ (k, v)) \in T'.ops$ 
45:        if  $op = R(k, v) \wedge int\_val[T'.tid][k] = \perp_v \wedge k \in keys$ 
46:          if  $ext\_val[tid][k] \neq v$ 
47:             $T'.EXT \leftarrow \perp$ 
48:          else
49:             $T'.EXT \leftarrow \top$ 
50:            if  $k \in keys$ 
51:               $int\_val[T'.tid][k] \leftarrow v$ 
52:            else  $\triangleright ts = T'.commit\_ts$ 
53:              for  $k \in Dom(int\_val[T'.tid])$ 
54:                 $int\_val[T'.tid][k] \leftarrow \perp_v$   $\triangleright$  reset int_val of  $T'$ 
55:               $keys \leftarrow keys \setminus T'.wkey$ 
56:              if  $keys = \emptyset$ 
57:                break
58:              for  $k \in keys$ 
59:                 $frontier\_ts[ts][k] \leftarrow ext\_val[tid][k]$ 
60:                 $ext\_val[tid] \leftarrow \emptyset$   $\triangleright$  gc ext_val of  $T$ 

61: procedure TIMEOUT( $T$ )  $\triangleright$  runs when timeout for  $T$  expires
62:   if  $T.EXT = \perp$ 
63:     report a violation of EXT
    $\triangleright$  gc frontier_ts, ongoing_ts, and transactions below timestamp  $ts$ 
64: procedure GARBAGECOLLECT( $ts$ )  $\triangleright$  runs periodically
65:   for  $ts' \leq ts$ 
66:      $frontier\_ts[ts'] \leftarrow \emptyset$   $\downarrow$ 
67:      $ongoing\_ts[ts'] \leftarrow \emptyset$   $\downarrow$ 
68:      $\mathcal{T} \leftarrow \mathcal{T} \setminus \{T \in \mathcal{T} \mid T.commit\_ts \leq ts\}$   $\downarrow$ 

```

---

as  $\uparrow$ ). AION reloads these data structures and transactions as needed later on (refer to code lines marked as  $\uparrow$ ).

**3.3.4 Complexity Analysis.** AION behaves similarly to CHRONOS in terms of complexity for (re-)checking the SESSION, INT, EXT, and NoCONFLICT axioms when a new transaction is received. However, instead of sorting transactions based on their timestamps *a priori* as in CHRONOS, AION inserts the new transaction into an already sorted list of transactions, which can be done in logarithmic time using, for example, balanced binary search trees. Therefore, the time complexity of AION for each new transaction is  $O(\log N + M)$ , where  $N$  is the number of transactions received so far, and  $M$  is the number of operations in the transactions.

The space complexity of AION is primarily determined by the memory required for storing the ever-growing history, as well as the versioned frontier\_ts and ongoing\_ts data structures. Thanks to its garbage collection mechanism, when asynchrony is minimal, AION only needs to keep in memory a few recent transactions and recent versions of frontier\_ts and ongoing\_ts.

## 4 EXPERIMENTS ON CHRONOS

In this section, we evaluate the offline checking algorithm CHRONOS and answer the following questions:

- (1) How efficient is CHRONOS, and how much memory does it consume? Can CHRONOS outperform the state of the art under various workloads and scale up to large workloads?

**Table 1: Workload parameters.**

| Parameters                                      | Values                       | Default |
|-------------------------------------------------|------------------------------|---------|
| Number of sessions (#sess)                      | 10, 20, 50, 100, 200         | 50      |
| Number of transactions (#txns)                  | 5K, 100K, 200K, 500K, 1,000K | 100K    |
| Number of operations per transaction (#ops/txn) | 5, 15, 30, 50, 100           | 15      |
| Ratio of read operations (%reads)               | 10%, 30%, 50%, 70%, 90%      | 50%     |
| Number of keys (#keys)                          | 200, 500, 1000, 2000, 5000   | 1000    |
| Distribution of key access (dist)               | Uniform, Zipfian, Hotspot    | Zipfian |

- (2) How do the individual components contribute to CHRONOS’s performance? Particularly, what impact does GC have on CHRONOS’s efficiency and memory usage?

#### 4.1 Performance and Scalability

We conduct a comprehensive performance analysis of CHRONOS and compare it to four other SI checkers under various workloads:

- PolySI [19] is an SI checker designed for key-value histories. It characterizes SI using (generalized) polygraphs [12, 23, 29], encodes the constraints on the polygraph as SMT clauses, and utilizes domain-specific optimizations and the MonoSAT [6] solver to efficiently check the acyclicity of the polygraph. PolySI has shown superior performance compared to dbcop [9] under various workloads [19].
- Viper [34] is also an SI checker for key-value histories. To capture the `begin` and `commit` timestamps in Adya’s formalization [4], Viper characterizes SI using **BC**-polygraphs. It also applies domain-specific optimizations and MonoSAT to efficiently check the acyclicity of the BC-polygraph.
- Elle [20] is a checker for various isolation levels, including SI. It can infer the transactional dependency efficiently and check SI in polynomial time on list histories. We also consider the Elle checker for key-value histories. We denote the two versions of Elle as ElleList and ElleKV, respectively.

**4.1.1 Workloads.** We tune the seven workload parameters, as shown in Table 1, during workload generation. The “Default” column presents the default values for these parameters. For the “hotspot” key-access distribution, we mean that 80% of operations target 20% of keys.

**4.1.2 Setup.** We evaluate all checkers using histories that *satisfy* SI. Specifically, we use histories collected from Dgraph (v20.03.1) operating on a key-value store. However, as Dgraph lacks support for list data types, we resort to histories collected from TiDB (v7.1.0) for comparing CHRONOS with ElleList. Both Dgraph and TiDB are deployed on a cluster of 3 machines in a local network. Two of these machines are equipped with a 2.545GHz AMD EPYC 7K83 (2-core) processor and 16GB memory, while the third machine has a 2.595GHz AMD EPYC 7K62 (16-core) processor and 64GB memory. Both CHRONOS and AION are deployed on the 16-core machine.

**4.1.3 Runtime and Scalability.** As shown in Figure 3, CHRONOS, as well as ElleKV, significantly outperforms PolySI and Viper on key-value histories, which exhibit super-linear growth with the number

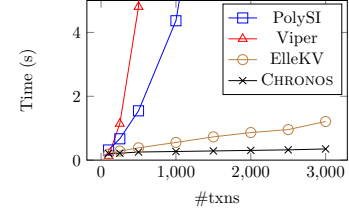

**Figure 3: Runtime comparison on key-value histories under varying number of transactions.**

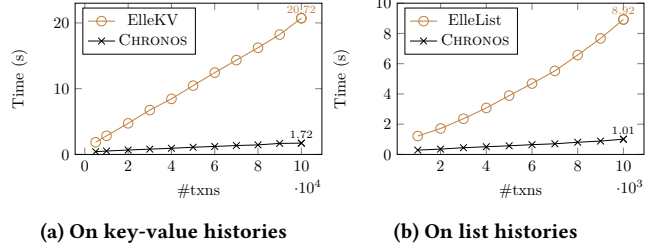

**Figure 4: Runtime comparison with ElleKV and ElleList under varying number of transactions.**

of transactions. To further compare CHRONOS with ElleKV on key-value histories and ElleList on list histories, we continue increasing the number of transactions and plot the runtime in Figure 4a and 4b, respectively. Similar to CHRONOS, the runtime of both ElleKV and ElleList grows (almost) linearly with the number of transactions. However, CHRONOS exhibits a much slower rate of growth because it processes transactions in their timestamp order and does not need to perform cycle detection like Elle. Specifically, CHRONOS is about 14.6 times faster than ElleKV and 10.7 times faster than ElleList. Remarkably, CHRONOS can check a key-value history with 100K transactions within 2 seconds (Figure 4a). Since list histories are more complex than key-value histories, CHRONOS requires a little more time to check them. For example, CHRONOS takes one second to check a list history with 10K transactions (Figure 4b).

We further investigate the impact of varying workload parameters on the performance of CHRONOS. The results shown in Figure 5 (see the line marked with  $\square$ ) align with our time complexity analysis in Section 3.2.3. Specifically, the runtime of CHRONOS increases (almost) linearly with both the total number of transactions per session (a) and the number of operations per transaction (b), while it remains stable concerning other parameters (c, d, e, f).

Figure 5a also illustrates that CHRONOS can check key-value histories containing up to 1 million transactions (with default values for other parameters) in about 17 seconds, showcasing its remarkable scalability. Conversely, PolySI takes several hours and Viper struggles to handle them effectively [19].

In Figure 5, we also explore the impact of varying GC frequencies on CHRONOS’s performance. In these experiments, we trigger GC periodically after processing a certain number of transactions (e.g., 10K and 500K), with ‘gc- $\infty$ ’ indicating that no GC is called at all. The results show that as GC is called more frequently, CHRONOS takes longer to check the history. Moreover, while the runtime shows

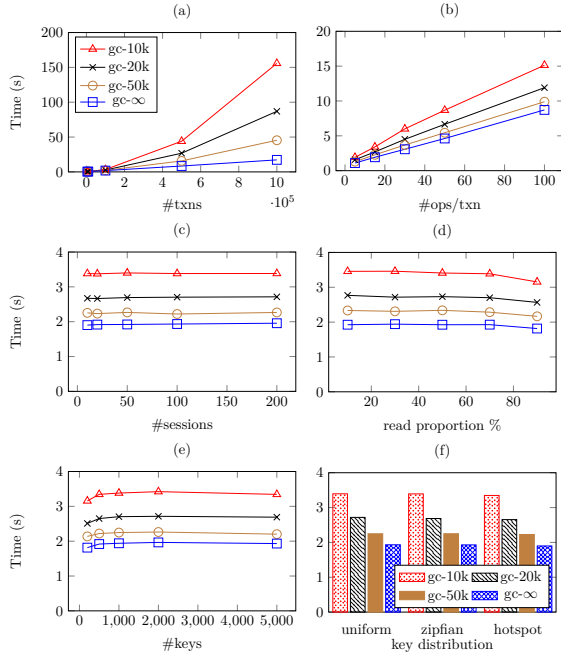

**Figure 5: Runtime of CHRONOS with various GC strategies under varying workload parameters.**

linear growth concerning the number of operations per transaction (b), the growth rate concerning the total number of transactions exceeds linearity when GC is called more frequently (a). This is because we tune the GC frequencies based on the number of transactions processed rather than the number of operations processed. In Section 4.2.1, we delve deeper into the time consumption of each stage of CHRONOS under varying GC frequencies.

**4.1.4 Memory Usage and Scalability.** As shown in Figure 6, the *maximum* memory usage of CHRONOS increases linearly with the number of transactions (a) and the number of operations per transaction (b), while it remains stable concerning other parameters (c, d, e, f). This aligns with our space complexity analysis in Section 3.2.3.

Figure 6a illustrates that CHRONOS consumes about 13 GB of memory when checking a key-value history with 1 million transactions. In contrast, both PolySI and Viper require significantly more memory to store the additional polygraph containing a large number of constraints when checking such large histories [19]. ElleKV also consumes much more memory than CHRONOS due to the extensive dependency graphs it constructs for histories [20].

## 4.2 A Closer Look at CHRONOS

**4.2.1 Runtime Decomposition of CHRONOS.** We measure CHRONOS’s checking time in terms of four stages:

- *loading* which loads the whole history into memory;
- *sorting* which sorts the start and commit timestamps of transactions in ascending order;
- *checking* which checks the history by examining axioms; and
- *garbage collecting* (GC) which recycles transactions that are no longer needed during checking.

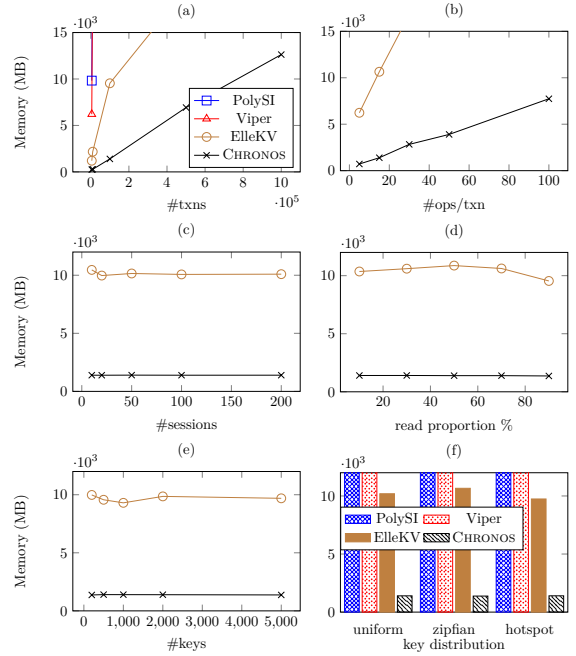

**Figure 6: The maximum memory usage under varying workload parameters.**

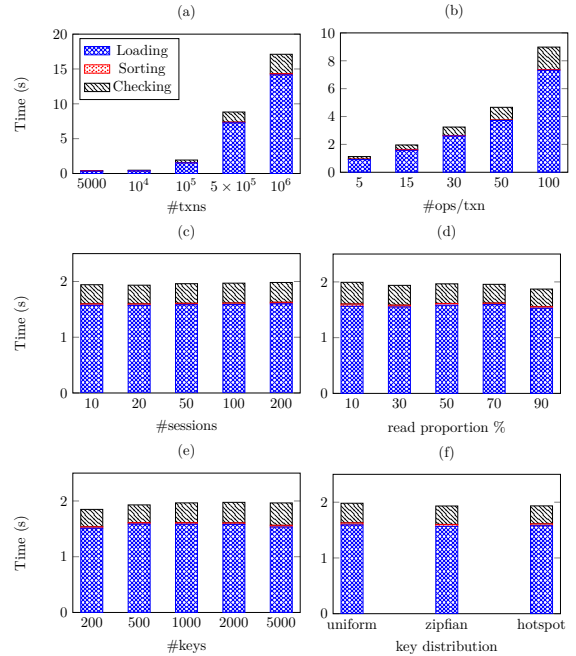

**Figure 7: Runtime decomposition of CHRONOS (without GC) under varying workload parameters.**

Figure 7 shows the time consumption of each stage of CHRONOS *without* GC under varying workload parameters. First, the loading stage, which involves frequent file I/O operations, is the most

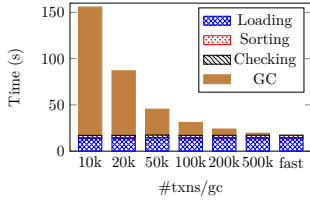

**Figure 8: Runtime decomposition of CHRONOS under varying GC frequencies.**

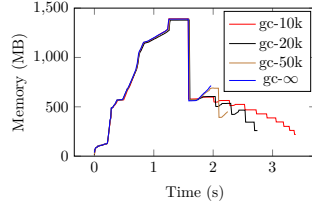

**Figure 9: Memory usage of CHRONOS over time.**

time-consuming, while the sorting stage (in memory) is negligible. Second, the time spent on both the loading and checking stages increases almost linearly with the total number of transactions (a) and the number of operations per transaction (b), while it remains stable concerning other parameters.

Figure 8 illustrates the impact of varying GC frequencies on the time consumption of each stage when checking a history of 1 million transactions. The results indicate that GC becomes the most time-consuming stage when it is called frequently. The time spent on GC decreases linearly as the GC frequency decreases.

**4.2.2 Memory Usage of CHRONOS over Time.** Figure 9 depicts the memory usage of CHRONOS over time when checking a key-value history of 100K transactions. Initially, the memory usage steadily increases until reaching its peak during the loading stage. Subsequently, a sharp decline occurs in memory usage due to a JVM GC before checking. During the checking stage, the memory usage displays a sawtooth pattern, characterized by intermittent increases followed by decreases after each (CHRONOS) GC. Overall, the memory usage gradually decreases over time until the checking stage ends. It is observed that more frequent GC calls result in smaller memory releases per GC and longer total runtime. Therefore, GC should be called judiciously in the offline checking stage.

## 5 EXPERIMENTS ON AION

In this section, we evaluate the online checking algorithm AION and answer the following questions:

- (1) What is the throughput that AION can achieve? How does AION perform with constrained memory resources?
- (2) How does the asynchronous arrival of transaction affect the stability of detecting the EXT violations?
- (3) How does the overhead of collecting histories affect the throughput of database systems?

### 5.1 Setup

We generate transaction histories using the same workload described in Table 1. The setup of the database systems and the checkers are the same as those described in Section 4. The network bandwidth between the node hosting AION and the database instances is 20Mbps, with an average latency of approximately 0.2ms. History collectors dispatch transaction histories to AION every 500 transactions.

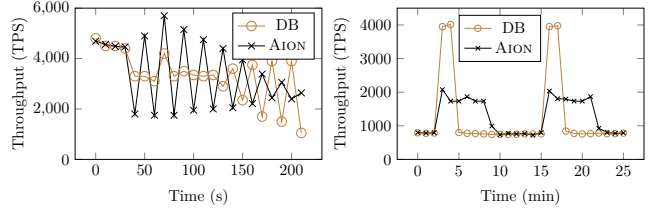

(a) In seconds

(b) In minutes

**Figure 10: Throughputs of both database and AION.**

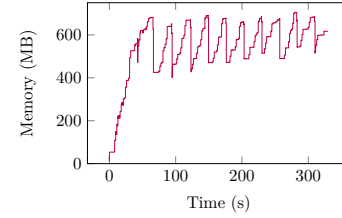

**Figure 11: Constrained memory usage of AION over time.**

### 5.2 Throughput

Figure 10 illustrates the throughput of AION alongside the database's throughput, measured in Transactions Per Second (TPS). In Figure 10(a), we set the number of operations per transaction to 8 to match the default setting of Cobra [29], an online checker for serializability (see Section 7 for comparison). The result demonstrates that AION can achieve a TPS of up to 4K. The throughput of AION has experienced some fluctuations due to periodic GC performed during the whole online checking stage. Nevertheless, the average TPS of AION in steady state is approximately 3K, sufficient to keep pace with the database's TPS. This indicates AION's capacity to effectively handle nearly 260 million transactions per day, approximately one third of the daily transaction volume of VISA's global payments and cash transactions in 2023 [2].

In Figure 10(b), while maintaining the database's peak TPS at 4K, we increase the number of operations per transaction to 15. As expected, AION's TPS drops to approximately 2K due to the (linearly) increased runtime and space complexity of the checking algorithm. AION can continually process transactions at its maximum capacity. As the database's TPS decreases, AION gradually catches up.

To evaluate the impact of memory constraints on AION, we mandate that AION triggers GC when memory usage surpasses 700M in the experiment depicted in Figure 11. This experiment is conducted using a workload comprising 100K transactions. We observe that AION initially consumes memory gradually until it reaches the maximum memory usage threshold. Subsequently, memory usage oscillates between 400M and 700M due to periodic GC, until the database finishes processing all transactions in approximately 310 seconds. Consequently, AION can effectively manage continuous online checking with relatively constrained memory resources.

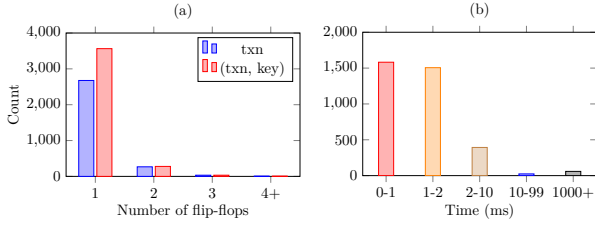

**Figure 12: The number of flip-flops and the time spent on rectifying the false positives/negatives. (The delays injected follow the normal distribution of  $N(100, 10^2)$ .)**

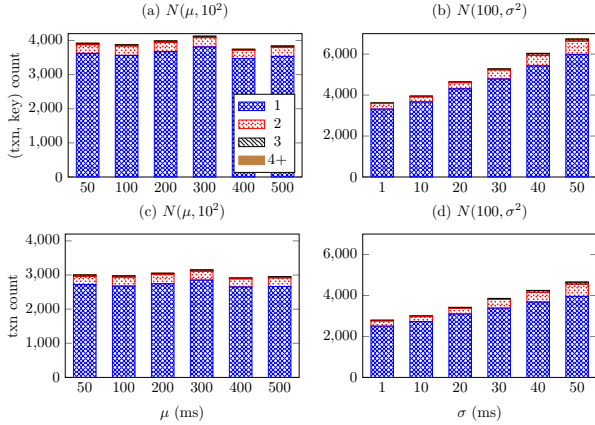

**Figure 13: Number of flip-flops (in terms of both (txn, key) count and txn count).**

### 5.3 Stability of Detecting the EXT Violations

We evaluate the impact of asynchrony on the stability of detecting the EXT violations by counting the number of flip-flops, denoting switches between  $T.EXT \leftarrow \top$  and  $T.EXT \leftarrow \perp$  for each transaction  $T$ . As the history collector delivers transactions to the checker in batches (500 transactions per batch), we introduce artificial random delays for each transaction within each batch, following a normal distribution, to mimic asynchrony. For these experiments, we utilize workloads consisting of 10K transactions.

An EXT violation manifests as a transaction-key pair. In Figure 12(a), the right bar denotes the number of EXT violations, while the left bar denotes the number of unique transactions (txn) involved in these violations. In these experiments, we inject delays following a normal distribution with a mean of 100 and a standard deviation of 10, i.e.,  $N(100, 10^2)$ . We observe that 29.8% of transactions exhibit flip-flops, with the majority (99%) experiencing them once or twice. Furthermore, Figure 12(b) reveals that over 95% of the false positives/negatives are rectified within 10 ms. Notably, approximately 3% of the false positives/negatives take about 1.5 seconds to be resolved, probably in the subsequent batch. Hence, setting a slightly higher time threshold for reporting violations than the batch latency would help mitigate the impact of these false positives/negatives.

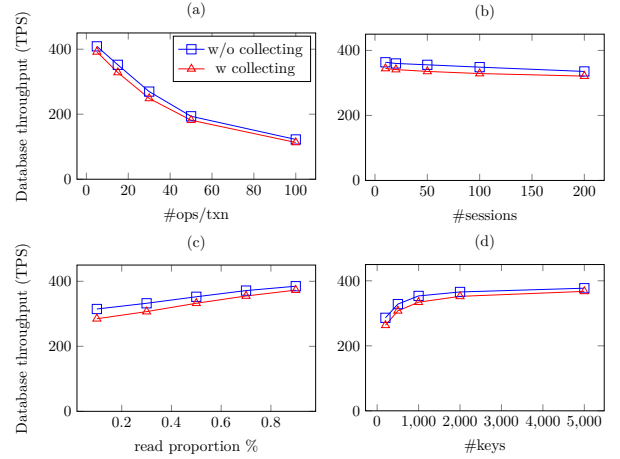

**Figure 14: Throughput with/without collecting history.**

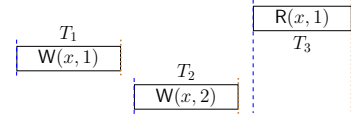

**Figure 15: A history that satisfies SI under traditional black-box SI checking but not under timestamp-based checking.**

As shown in Figure 13(a,c), the mean ( $\mu$ ) of delays has a negligible impact on the number of flip-flops since transactions have been equally deferred. Conversely, as shown in Figure 13(b,d), increasing the standard deviation ( $\sigma$ ) of delays leads to a higher number of flip-flops, due to the increased likelihood of transactions arriving out of order.

### 5.4 Overhead of Collecting Histories

Figure 14 compares the database throughputs with and without history collection, under a workload comprising 20K transactions. Across various parameters, we observe that collecting (and transmitting) the history leads to a roughly 5% decrease in TPS, indicating a minor impact.

## 6 DISCUSSIONS AND LIMITATIONS

*Completeness of Timestamp-based Checking.* The timestamp-based checking approach offers an additional advantage over the traditional black-box approach in terms of *completeness*. The latter might overlook SI violations in certain histories from the perspective of database developers. For instance, consider the scenario depicted in Figure 15, where transactions  $T_1$ ,  $T_2$ , and  $T_3$  are committed sequentially. Database developers envisioning the database's timestamp-based operational semantics might expect an SI violation, as  $T_3$  reads from a snapshot that excludes the effect of  $T_2$ . However, traditional black-box SI checkers accept this history as SI, falsely inferring an execution order, i.e.,  $T_1, T_3, T_2$ , which did not occur.

*On (Strict) Serializability Checking.* Our approach is also applicable to the serializability checking problem. The insight is that

databases that implement serializability aim to ensure that transactions appear to be executed in the increasing order of their commit timestamps. Implementing the timestamp-based checking approach and designing efficient checking algorithms for serializability are generally simpler compared to those for snapshot isolation.

A number of databases, such as Google Spanner [14, 15], FoundationDB [35], and FaunaDB [18], have implemented strict serializability [4]. Checking strict serializability in our approach entails accessing the *wall-clock* start and commit timestamps of each transaction. We will explore how to faithfully obtain these timestamps.

*Data Types and Queries.* Our approach is general and adaptable regardless of the data types and query languages used to generate the histories. We anticipate that extending CHRONOS and AION to accommodate more data types such as sets, queues, and JSON documents, along with intricate queries like SQL range queries, SQL Join operator, and graph path queries, will be more feasible compared to other black-box checkers.

*Limitations.* To our knowledge, centralized databases like SQL Server [26], PostgreSQL [25], and WiredTiger [3] implement SI in a similar manner, without relying on timestamp-based mechanisms. They associate each transaction with a unique identifier, but the transaction identifiers, such as those used in WiredTiger, may not directly correlate with the timestamps employed in the database systems considered in this paper. For instance, transactions are not necessarily committed in the order of their identifiers. Moreover, conditions like  $T_1.tid < T_2.tid$  and  $T_2$  being visible to  $T_3$  do not necessarily imply that  $T_1$  is also visible to  $T_3$ . Thus, they utilize a *visibility rule* to compute the snapshot of a transaction, i.e., the *set* of transaction identifiers visible to it. We plan to extend our approach to handle such databases, and further, to formally specify and verify these SI implementations in our future work.

## 7 RELATED WORK

It is known that the SI checking problem is NP-complete for general key-value histories where the transaction execution order is unknown, even under the UniqueValue assumption [9]. Existing SI checkers fall into two categories: those designed for general histories and those tailored for histories with additional information.

*Checkers for General Histories.* The SI checking algorithms proposed in [9] are polynomial time assuming that certain input history parameters, e.g., the number of sessions, are fixed. However, they lack practical efficiency as these fixed parameters can be large [19]. PolySI [19], influenced by both Cobra [29] for serializability checking and the characterization of SI using dependency graphs [12], encoded the SI checking problem into an SMT problem, seeking cycles in a generalized polygraph [23, 29], and then resolves it using the MonoSAT solver [6]. Viper [34] introduces BC-polygraphs as a new representation of transactional dependencies, reduces the SI checking problem into a cycle detection problem on BC-polygraphs, and leverages MonoSAT to solve it. Essentially, these checkers need to explore all potential transaction execution orders, and their computational cost grows exponentially with the number  $N$  of transactions in the history in the worst case. In contrast, our offline checking algorithm CHRONOS costs  $O(N \log N + M)$  time, where  $M$  is the number of operations in the history.

*Checkers for Histories with Additional Information.* Elle [20] can infer the transaction execution order in a history (more precisely, the version order of a history in Adya’s formalism [4]) by carefully choosing data types and utilizing the UniqueValue assumption to generate recoverable and traceable histories. Elle scales well to histories with tens of thousands of transactions, but struggles with those containing hundreds of thousands of transactions due to expensive cycle detection performed on extensive dependency graphs of such large histories. Elle works well for data types such as lists, but for some data types such as read-write registers (i.e., key-value pairs), counters, and sets, it can make only limited inferences. In contrast, our checking algorithms leverage timestamps to infer the transaction execution order. They are neither limited to specific data types nor to the UniqueValue assumption.

When the start and commit timestamps of transactions are available in some snapshot-isolated database systems, Elle [20] can utilize them to infer the time-precedes order among transactions in Adya’s formalism of SI and construct a start-ordered serialization graph [4]. In our timestamp-based approach, we infer the transaction execution order according to their commit timestamps and check the SI axioms on the fly while simulating the execution of transactions one by one, without constructing extensive dependency graphs and performing expensive cycle detection on them.

Clark et al. [13] introduced the concept of version order recovery, similar to the notion of traceability in Elle. They demonstrated that the version order of a history can be easily recovered from PostgreSQL and TiDB, utilizing their CDC mechanism. Additionally, they designed an efficient serializability checker based on version order recovery. In contrast, our checking algorithms focus on SI, for which inferring the snapshot of each transaction is also essential.

To our knowledge, none of the existing checkers, unlike our AION, supports online checking for SI. Cobra [29] is the only checker that supports online checking for serializability, claiming a throughput of 2k TPS with GPU acceleration on workloads featuring 8 operations per transaction. However, Cobra needs to inject “fence transactions” into client workloads, which is often unacceptable in production. Furthermore, our offline checker CHRONOS significantly outperforms PolySI (Section 4), which has been demonstrated to be faster than Cobra [19].

## 8 CONCLUSION AND FUTURE WORK

We have proposed a timestamp-based approach to checking snapshot isolation (SI) in database systems. By leveraging the start and commit timestamps of transactions in a history, we can infer the transaction execution order and determine the snapshot of each transaction. We have developed both offline and online highly efficient SI checking algorithms, named CHRONOS and AION, respectively. Our algorithms are not restricted to specific data types or the UniqueValue assumption.

We plan to extend CHRONOS and AION to accommodate more data types and complex queries such as SQL range queries and graph path queries. To further improve the scalability of AION, we will explore techniques to parallelize the checking process and leverage multi-core processors and GPUs. Finally, we will investigate how to adapt our approach to check both serializability and strict serializability in database systems.

## REFERENCES

- [1] 2024. Chronos and Aion: Offline and Online Timestamp-based Checking of Snapshot Isolation in Database Systems. <https://anonymous.4open.science/r/TimeKiller-660D/>.
- [2] Accessed April, 2024. VISA Fact Sheet. <https://usa.visa.com/dam/VCOM/global/about-visa/documents/aboutvisafactsheet.pdf>.
- [3] Accessed April, 2024. WiredTiger (Version 10.0.2): Snapshot. <http://source.wiredtiger.com/mongodb-5.0/arch-snapshot.html>.
- [4] Atul Adya. 1999. *Weak Consistency: A Generalized Theory and Optimistic Implementations for Distributed Transactions*. Ph. D. Dissertation. USA.
- [5] Peter Bailis, Aaron Davidson, Alan Fekete, Ali Ghodsi, Joseph M. Hellerstein, and Ion Stoica. 2013. Highly Available Transactions: Virtues and Limitations. *Proc. VLDB Endow.* 7, 3 (nov 2013), 181–192. <https://doi.org/10.14778/2732232.2732237>
- [6] Sam Bayless, Noah Bayless, Holger H. Hoos, and Alan J. Hu. 2015. SAT modulo Monotonic Theories. In *Proceedings of the Twenty-Ninth AAAI Conference on Artificial Intelligence (AAAI’15)*. AAAI Press, 3702–3709.
- [7] Hal Berenson, Phil Bernstein, Jim Gray, Jim Melton, Elizabeth O’Neil, and Patrick O’Neil. 1995. A Critique of ANSI SQL Isolation Levels. In *SIGMOD ’95*. ACM, 1–10. <https://doi.org/10.1145/223784.223785>
- [8] Philip A Bernstein, Vassos Hadzilacos, and Nathan Goodman. 1986. *Concurrency Control and Recovery in Database Systems*. Addison-Wesley Longman Publishing Co., Inc., USA.
- [9] Ranadeep Biswas and Constantin Enea. 2019. On the Complexity of Checking Transactional Consistency. *Proc. ACM Program. Lang.* 3, OOPSLA, Article 165 (Oct. 2019), 28 pages. <https://doi.org/10.1145/3360591>
- [10] Ranadeep Biswas, Diptanshu Kakwani, Jyothi Vedurada, Constantin Enea, and Akash Lal. 2021. MonkeyDB: Effectively Testing Correctness under Weak Isolation Levels. *Proc. ACM Program. Lang.* 5, OOPSLA, Article 132 (oct 2021), 27 pages. <https://doi.org/10.1145/3485546>
- [11] Andrea Cerone, Giovanni Bernardi, and Alexey Gotsman. 2015. A Framework for Transactional Consistency Models with Atomic Visibility. In *CONCUR’15 (LIPIcs, Vol. 42)*. Schloss Dagstuhl–Leibniz-Zentrum fuer Informatik, 58–71.
- [12] Andrea Cerone and Alexey Gotsman. 2018. Analysing Snapshot Isolation. *J. ACM* 65, 2, Article 11 (Jan. 2018), 41 pages. <https://doi.org/10.1145/3152396>
- [13] Jack Clark. 2021. *Verifying Serializability Protocols With Version Order Recovery*. Master’s thesis. ETH Zurich. <https://doi.org/10.3929/ethz-b-000507577>.
- [14] James C. Corbett, Jeffrey Dean, Michael Epstein, Andrew Fikes, Christopher Frost, J. J. Furman, Sanjay Ghemawat, Andrey Gubarev, Christopher Heiser, Peter Hochschild, Wilson Hsieh, Sebastian Kanthak, Eugene Kogan, Hongyi Li, Alexander Lloyd, Sergey Melnik, David Mwaura, David Nagle, Sean Quinlan, Rajesh Rao, Lindsay Rolig, Yasushi Saito, Michal Szymaniak, Christopher Taylor, Ruth Wang, and Dale Woodford. 2012. Spanner: Google’s Globally-Distributed Database. In *Proceedings of the 10th USENIX Conference on Operating Systems Design and Implementation (OSDI’12)*. USENIX Association, USA, 251–264.
- [15] James C. Corbett, Jeffrey Dean, Michael Epstein, Andrew Fikes, Christopher Frost, J. J. Furman, Sanjay Ghemawat, Andrey Gubarev, Christopher Heiser, Peter Hochschild, Wilson Hsieh, Sebastian Kanthak, Eugene Kogan, Hongyi Li, Alexander Lloyd, Sergey Melnik, David Mwaura, David Nagle, Sean Quinlan, Rajesh Rao, Lindsay Rolig, Yasushi Saito, Michal Szymaniak, Christopher Taylor, Ruth Wang, and Dale Woodford. 2013. Spanner: Google’s Globally Distributed Database. *ACM Trans. Comput. Syst.* 31, 3, Article 8 (aug 2013), 22 pages. <https://doi.org/10.1145/2491245>
- [16] Khuzaima Daudjee and Kenneth Salem. 2006. Lazy Database Replication with Snapshot Isolation. In *VLDB’06*. VLDB Endowment, 715–726.
- [17] Dgraph. Accessed April, 2024. <https://dgraph.io/>.
- [18] FaunaDB. Accessed April, 2024. Fauna’s Distributed Transaction Engine (DTE). <https://fauna.com/distributed-transaction-engine>.
- [19] Kaile Huang, Si Liu, Zheng Chen, Hengfeng Wei, David Basin, Haixiang Li, and Anqun Pan. 2023. Efficient Black-Box Checking of Snapshot Isolation in Databases. *Proc. VLDB Endow.* 16, 6 (apr 2023), 1264–1276. <https://doi.org/10.14778/3583140.3583145>
- [20] Kyle Kingsbury and Peter Alvaro. 2020. Elle: Inferring Isolation Anomalies from Experimental Observations. *Proc. VLDB Endow.* 14, 3 (Nov. 2020), 268–280.
- [21] Memgraph. Accessed April, 2024. <https://memgraph.com/>.
- [22] MongoDB. Accessed April, 2024. <https://www.mongodb.com/>.
- [23] Christos H. Papadimitriou. 1979. The Serializability of Concurrent Database Updates. *J. ACM* 26, 4 (oct 1979), 631–653. <https://doi.org/10.1145/322154.322158>
- [24] Daniel Peng and Frank Dabek. 2010. Large-Scale Incremental Processing Using Distributed Transactions and Notifications. In *OSDI’10*. USENIX Association, USA, 251–264.
- [25] PostgreSQL. Accessed April, 2024. Database Concurrency in PostgreSQL. <https://www.red-gate.com/simple-talk/databases/postgresql/database-concurrency-in-postgresql/>.
- [26] Microsoft SQL Server. Accessed April, 2024. Snapshot Isolation in SQL Server. <https://learn.microsoft.com/en-us/dotnet/framework/data/adonet/sql/snapshot-isolation-in-sql-server>.
- [27] Ohad Shacham, Francisco Perez-Sorrosal, Edward Bortnikov, Eshcar Hillel, Idit Keidar, Ivan Kelly, Matthieu Morel, and Sameer Paranjpye. 2017. Omid, reloaded: scalable and highly-available transaction processing. In *Proceedings of the 15th Usenix Conference on File and Storage Technologies (Santa clara, CA, USA) (FAST’17)*. USENIX Association, USA, 167–180.
- [28] Yair Sovran, Russell Power, Marcos K. Aguilera, and Jinyang Li. 2011. Transactional Storage for Geo-Replicated Systems. In *SOSP ’11*. ACM, 385–400. <https://doi.org/10.1145/2043556.2043592>
- [29] Cheng Tan, Changgeng Zhao, Shuai Mu, and Michael Walfish. 2020. COBRA: Making Transactional Key-Value Stores Verifiably Serializable. In *OSDI’20*. Article 4, 18 pages.
- [30] Jepsen testing of MongoDB 4.2.6. Accessed April, 2024. <http://jepsen.io/analyses/mongodb-4.2.6>.
- [31] Jepsen testing of TiDB 2.1.7. Accessed April, 2024. <https://jepsen.io/analyses/tidb-2.1.7>.
- [32] TiDB. Accessed April, 2024. <https://en.pingcap.com/tidb/>.
- [33] YugabyteDB. Accessed April, 2024. <https://www.yugabyte.com/>.
- [34] Jian Zhang, Ye Ji, Shuai Mu, and Cheng Tan. 2023. Viper: A Fast Snapshot Isolation Checker. In *Proceedings of the Eighteenth European Conference on Computer Systems (Rome, Italy) (EuroSys ’23)*. Association for Computing Machinery, New York, NY, USA, 654–671. <https://doi.org/10.1145/3552326.3567492>
- [35] Jingyu Zhou, Meng Xu, Alexander Shraer, Bala Namasivayam, Alex Miller, Evan Tschannen, Steve Atherton, Andrew J. Beamon, Rusty Sears, John Leach, Dave Rosenthal, Xin Dong, Will Wilson, Ben Collins, David Scherer, Alec Grieser, Young Liu, Alvin Moore, Bhaskar Muppana, Xiaoge Su, and Vishesh Yadav. 2021. FoundationDB: A Distributed Unbundled Transactional Key Value Store. In *Proceedings of the 2021 International Conference on Management of Data (SIGMOD ’21)*. Association for Computing Machinery, New York, NY, USA, 2653–2666. <https://doi.org/10.1145/3448016.3457559>
