# Supplementary material for: Online Timestamp-based Transactional Isolation Checking of Database Systems (Extended Version)
Source: arXiv:2504.01477 source file (2025-04-02)
Supplement: Supplementary file 6 [file si-impl.tex]

% si-impl.tex

\begin{table*}[t]
	\centering
	\caption{Timestamp-based implementation of snapshot isolation in databases.}
	\label{table:si-impl}
	
	\resizebox{0.80\textwidth}{!}{%
		\begin{tabular}{|c|c|c|c|c|c|c|c|c|}
		\hline
		DBMS & Data Model & GitHub Stars & Timestamping & Timestamps & $\starttime$ & $\committime$ & Reference & Confirmed \\ \hline
		\hline
		MongoDB		&      &        &        &            &              &               &           &           \\ \hline
		TiDB	&      &        &        &            &              &               &           &           \\ \hline
		YugabyteDB	&      &        &        &            &              &               &           &           \\ \hline
		Dgraph	&      &        &        &            &              &               &           &           \\ \hline
				&      &        &        &            &              &               &           &           \\ \hline
		\end{tabular}%
	}
\end{table*}
