# Supplementary material for: Online Timestamp-based Transactional Isolation Checking of Database Systems (Extended Version)
Source: arXiv:2504.01477 source file (2025-04-02)
Supplement: Supplementary file 7 [file si-violations-known.tex]

% si-violations-known.tex

\begin{table}[t]
	\centering
	\caption{Known SI violations reproduced by \tool.}
	\label{table:si-violations-known}
  
  \resizebox{0.85\columnwidth}{!}{%
		\begin{tabular}{|c|c|c|}
			\hline
			{\bf Database} & {\bf Release} & {\bf Known SI Violations} \\ \hline\hline
			MongoDB & & \\ \hline
			TiDB & & \\ \hline
			YugabyteDB & & \\ \hline
			Dgraph & &  \\  \hline
		\end{tabular}
	}
\end{table}
