# Supplementary material for: Online Timestamp-based Transactional Isolation Checking of Database Systems (Extended Version)
Source: arXiv:2504.01477 source file (2025-04-02)
Supplement: Supplementary file 8 [file si-violations-new.tex]

% si-violations-new.tex

\begin{table}[t]
	\centering
	\caption{New SI violations found by \tool.}
	\label{table:si-violations-new}
  
  \resizebox{\columnwidth}{!}{%
		\begin{tabular}{|c|c|c|c|c|}
			\hline
			{\bf Database} & {\bf Release} & {\bf Known SI Violations} & {\bf Bug Report} & {\bf Status}
			\\ \hline\hline
			MongoDB & & & & \\ \hline
			TiDB & & & & \\ \hline
			YugabyteDB & & & & \\ \hline
			Dgraph & & & & \\ \hline
		\end{tabular}
	}
\end{table}
