# Supplementary material for: Online Timestamp-based Transactional Isolation Checking of Database Systems (Extended Version)
Source: arXiv:2504.01477 source file (2025-04-02)
Supplement: Supplementary file 10 [file chronos.tex]

% chronos.tex

% \small
\begin{algorithm}[t]
\footnotesize
	\caption{\tool: the offline SI checking algorithm}
	\label{alg:chronos}
	\begin{algorithmic}[1]
		\Statex $\lastsnoinsession \in \SID \to \N$:
		  $\sno$ of the last transaction already processed
			\Statex \quad in each session, initially $-1$
		\Statex $\lastctsinsession \in \SID \to \TS$:
		  $\committime$ of the last transaction already
			\Statex \quad processed in each session, initially $\nullts$

		% \hStatex
		\Statex $\frontier \in \Key \to \Val$:
			{the last committed value of each key, initially $\nullval$}
		\Statex $\ongoing \in \Key \to 2^{\TID}$:
		{the set of ongoing transactions on each key,}
			\Statex {\quad initially $\emptyset$}

		% \hStatex
		\Statex $\intval \in \TID \to (\Key \to \Val)$:
			the last read/written value of each key
				\Statex \quad in each transaction, {initially $\nullval$}

		\Statex $\extval \in \TID \to (\Key \to \Val)$:
			the last written value of each key
				\Statex \quad in each transaction, {initially $\nullval$}

		\hStatex
		\Procedure{\checksi}{$\H$} \Comment{$\H$ contains
		  the initial transaction $\nulltxn$}
			\label{line:proc-checksi}
			% \State add the initial transaction $\nulltxn$ to $\H$
			%    \label{line:checksi-init-so}

			\State sort $\TS$ in ascending order
				\label{line:checksi-sort-ts}

			\For{$\tsvar \in \TS$}
				\label{line:checksi-foreach-ts}
				\State $T \gets \text{ the transaction that owns the timestamp } \tsvar$
					\label{line:checksi-t}
				\State $\sid \gets T.\sid$ \qquad $\tid \gets T.\tid$
				  \qquad $T.\wkey \gets \emptyset$
				  \label{line:checksi-sid-tid}
					\label{line:checksi-t-wkey}

				\hStatex
				\If{$\tsvar = T.\starttime$} \Comment{start event of $T$}
				  \label{line:checksi-ts-startts}
					\If{{$T.\sno \neq \lastsnoinsession[\sid] + 1
					       \lor T.\starttime < \lastctsinsession[\sid]$}}
						\label{line:checksi-sessionaxiom-begin}
						\State {\it report a violation of \sessionaxiom}
					\EndIf
					\State $\lastsnoinsession[\sid] \gets T.\sno$
					\State $\lastctsinsession[\sid] \gets T.\committime$
						\label{line:checksi-sessionaxiom-end}

					\hStatex
					\For{$(\opvar = \_(k, v)) \in T.\ops$}
						\Comment{in program order}
						\If{$\opvar = \readevent(k, v)$}
							\label{line:checksi-rop}
							\label{line:checksi-intext-begin}
							\If{$\intval[\tid][k] = \nullval$}
								\Comment{external read}
								\label{line:checksi-ext-read}
								\If{{$v \neq \frontier[k]$}}
									\State {\it report a violation of \extaxiom}
									\label{line:checksi-extaxiom-violation}
								\EndIf
							\ElsIf {$\intval[\tid][k] \neq v$}
								\Comment{internal read}
								\label{line:checksi-int-read}
								\State {\it report a violation of \intaxiom}
								\label{line:checksi-intaxiom-violation}
							\EndIf
							\label{line:checksi-intext-end}
						\Else	\Comment{$\opvar = \writeevent(k, v)$}
							\label{line:checksi-wop}
							\label{line:checksi-wop-begin}
							\State $T.\wkey \gets T.\wkey \cup \set{k}$
								\label{line:checksi-wkey-k}
							\State $\extval[\tid][k] \gets v$
								\label{line:checksi-ext-wkey}
							\State {{{$\ongoing[k] \gets \ongoing[k] \cup \set{\tid}$}}}
								\label{line:checksi-ongoing-t-cup}
								\label{line:checksi-wop-end}
						\EndIf
						\State $\intval[\tid][k] \gets v$
							\label{line:checksi-intval}
					\EndFor
				\Else \Comment{commit event of $T$}
				  \label{line:checksi-ts-committs}
					\If{{$T.\starttime > T.\committime$}}
					  \label{line:checksi-startts-committs-begin}
						\Comment{{check Eq. (\ref{eq:si-startts-committs})}}
						\State {\it report an error}
							\label{line:checksi-startts-committs-end}
					\EndIf
					\For{$k \in T.\wkey$}
					  \label{line:checksi-each-k}
						\State $\ongoing[k] \gets \ongoing[k] \setminus \set{\tid}$
						  \Comment{except $T$ itself}
							\label{line:checksi-ongoing-t-setminus}
						\label{line:checksi-noconflictaxiom-begin}
							\If{$\ongoing[k] \neq \emptyset$}
								\label{line:checksi-noconflictaxiom-conflict}
								\State {\it report a violation of \noconflictaxiom}
								\label{line:checksi-noconflictaxiom-violation}
								\label{line:checksi-noconflictaxiom-end}
							\EndIf
							\State $\frontier[k] \gets \extval[\tid][k]$
								\label{line:checksi-frontier-k}
					\EndFor
					% \State $\gcstyle{T.\wkey \gets \emptyset}$
					%   \Comment{gc $\wkey$}
					% 	\label{line:checksi-gc-wkey}
						\label{line:checksi-gc-begin}
					\State $\gcstyle{\intval[\tid] \gets \emptyset}$
						\label{line:checksi-gc-intval}
						\Comment{gc $\intval$}
					\State $\gcstyle{\extval[\tid] \gets \emptyset}$
						\label{line:checksi-gc-extval}
						\Comment{gc $\extval$}
					\State $\gcstyle{\T \gets \T \setminus \set{T}}$
					  \label{line:checksi-gc-txn}
						\Comment{gc $T$}
						\label{line:checksi-gc-end}
				\EndIf
			\EndFor
		\EndProcedure
	\end{algorithmic}
\end{algorithm}
\normalsize
