# Supplementary material for: Online Timestamp-based Transactional Isolation Checking of Database Systems (Extended Version)
Source: arXiv:2504.01477 source file (2025-04-02)
Supplement: Supplementary file 11 [file si.tex]

% si.tex

\small
\begin{algorithm}[t]
  \caption{Operational Semantics of Snapshot Isolation}
  \label{alg:si}
  % \begin{varwidth}[t]{0.46\textwidth}
  \begin{algorithmic}[1]
		\Statex $\log$: the log of committed transactions

		\hStatex
    \Procedure{\starttxn}{$T$}
      \label{line:proc-starttxn}
			\State $T.\starttime \gets \timestamprequest(\timeoracle)$
			  \label{line:starttxn-starttime}
			\State \Return \ok
    \EndProcedure

		\hStatex
    \Procedure{\writetxn}{$T, k, v$}
      \label{line:proc-writetxn}
			\State $T.\buffer \gets T.\buffer \circ \tuple{k, v}$
			  % \Comment{append $\tuple{k, v}$ to $T.\buffer$}
			  \label{line:writetxn-buffer}
			\State \Return \ok
    \EndProcedure

		\hStatex
    \Procedure{\readtxn}{$T, k$}
      \label{line:proc-readtxn}
			\State \Return value of $k$ from $T.\buffer$
			  and $\log$ as of $T.\starttime$
				\label{line:readtxn-value}
    \EndProcedure

		\hStatex
    \Procedure{\committxn}{$T$}
      \label{line:proc-committxn}
			\State $T.\committime \gets \timestamprequest(\timeoracle)$
			  \label{line:committxn-committime}
			\If{$T$ \emph{conflicts} with some concurrent transaction}
			  \label{line:committxn-conflict-checking}
			  \State \Return $\aborted$
					\label{line:aborttxn-status}
			\EndIf
			\State $\log \gets \log \circ \tuple{T.\buffer, T.\committime}$
				% \Comment{append $T$ to $\log$}
				\label{line:committxn-log}
			\State \Return $\committed$
			  \label{line:committxn-return-status}
    \EndProcedure
  \end{algorithmic}
  % \end{varwidth}
\end{algorithm}
\normalsize
