# Supplementary material for: Online Timestamp-based Transactional Isolation Checking of Database Systems (Extended Version)
Source: arXiv:2504.01477 source file (2025-04-02)
Supplement: Supplementary file 15 [file exp-decompose-freq-and-memory-default.tex]

% exp-decompose-freq-and-memory-default.tex

\begin{figure}[t]
	\begin{minipage}{0.23\textwidth}
		\centering
		\includegraphics[width = 1\textwidth]{figs/exp-decompose-freq}
		\caption{Runtime decomposition of \tool{} under varying GC frequencies.}
		\label{fig:decompose-freq}
	\end{minipage}
	\hfill
	\begin{minipage}{0.23\textwidth}
		\centering
		\includegraphics[width = 1\textwidth]{figs/exp-memory-default}
		\caption{Memory usage of \tool{} over time.}
		\label{fig:memory-default}
	\end{minipage}
\end{figure}
