# Supplementary material for: Online Timestamp-based Transactional Isolation Checking of Database Systems (Extended Version)
Source: arXiv:2504.01477 source file (2025-04-02)
Supplement: Supplementary file 16 [file exp-decompose-freq.tex]

\begin{figure}[t]
	\centering
	\includegraphics[width = 0.4\textwidth]{figs/exp-decompose-freq}
	\caption{Time of each stage as GC frequency changes}
	\label{fig:decompose-freq}
\end{figure}
