# Supplementary material for: Online Timestamp-based Transactional Isolation Checking of Database Systems (Extended Version)
Source: arXiv:2504.01477 source file (2025-04-02)
Supplement: Supplementary file 18 [file exp-decompose.tex]

% exp-decompose.tex

\begin{figure}[t]
	\centering
	\includegraphics[width = 0.42\textwidth]{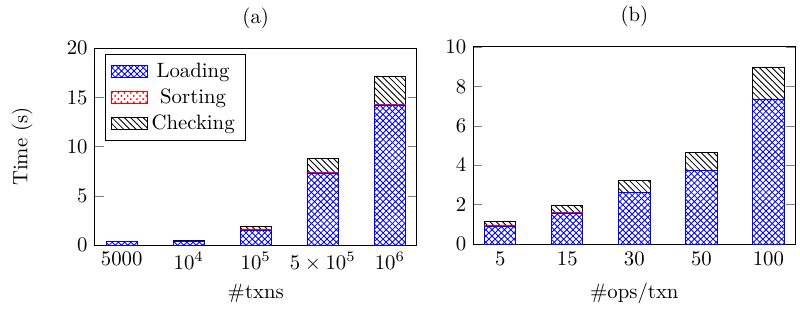}
	\caption{Runtime decomposition of \tool{} (without GC)
	  under varying workload parameters. }
	\label{fig:decompose}
\end{figure}
