# Supplementary material for: Online Timestamp-based Transactional Isolation Checking of Database Systems (Extended Version)
Source: arXiv:2504.01477 source file (2025-04-02)
Supplement: Supplementary file 19 [file exp-memory-default.tex]

% exp-memory-default.tex

\begin{figure}[t]
	\centering
	\includegraphics[width = 0.4\textwidth]{figs/exp-memory-default}
	\caption{Memory usage over time with default parameters}
	\label{fig:memory-default}
\end{figure}
