# Supplementary material for: Online Timestamp-based Transactional Isolation Checking of Database Systems (Extended Version)
Source: arXiv:2504.01477 source file (2025-04-02)
Supplement: Supplementary file 23 [file exp-online-flip-compact.tex]

\begin{figure}[t]
	\centering
	\includegraphics[width = 0.45\textwidth]{figs/exp-online-flip-compact-simplified.pdf}
  \caption{Number of flip-flops (in terms of (txn, key) count). }
	\label{fig:online-flip-compact}
    \vspace{-0.5cm}
\end{figure}
