# Supplementary material for: Online Timestamp-based Transactional Isolation Checking of Database Systems (Extended Version)
Source: arXiv:2504.01477 source file (2025-04-02)
Supplement: Supplementary file 27 [file exp-online-flip-time-sigma.tex]

\begin{figure}[t]
	\centering
	\includegraphics[width = 0.45\textwidth]{figs/exp-online-flip-time-sigma}
	\caption{Time to finalize the result of checking \extaxiom{} under varying standard deviations of delays.}
	\label{fig:online-flip-time-sigma}
\end{figure}
