# Supplementary material for: Online Timestamp-based Transactional Isolation Checking of Database Systems (Extended Version)
Source: arXiv:2504.01477 source file (2025-04-02)
Supplement: Supplementary file 29 [file exp-online-gc.tex]

% exp-online-gc.tex

\begin{figure}[t]
	\centering
	\includegraphics[width = 0.30\textwidth]{figs/exp-online-gc}
	\caption{Memory usage over time}
	\label{fig:online-gc}
\end{figure}
