# Supplementary material for: Online Timestamp-based Transactional Isolation Checking of Database Systems (Extended Version)
Source: arXiv:2504.01477 source file (2025-04-02)
Supplement: Supplementary file 30 [file exp-online-throughput-collection.tex]

\begin{figure}[t]
	\centering
	\includegraphics[width = 0.26\textwidth]{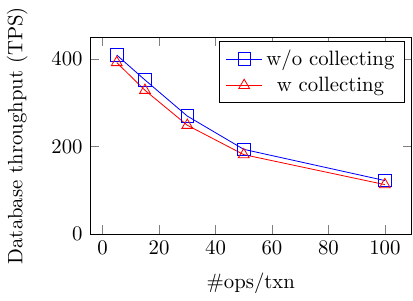}
	\caption{Database throughputs with and without collecting history.}
	\label{fig:exp-online-throughput-ops}
\end{figure}
