# Supplementary material for: Online Timestamp-based Transactional Isolation Checking of Database Systems (Extended Version)
Source: arXiv:2504.01477 source file (2025-04-02)
Supplement: Supplementary file 31 [file exp-online-throughput-memory.tex]

\begin{figure}[t]
	\centering
	\includegraphics[width = 0.25\textwidth]{figs/exp-online-gc}
	\caption{Constrained memory usage of \onlinetool{} over time.}
	\label{fig:exp-online-throughput-memory}
\end{figure}
