# Supplementary material for: Online Timestamp-based Transactional Isolation Checking of Database Systems (Extended Version)
Source: arXiv:2504.01477 source file (2025-04-02)
Supplement: Supplementary file 32 [file exp-online-throughput-ops-and-gc.tex]

\begin{figure}[t]
	\begin{minipage}{0.23\textwidth}
		\centering
		\includegraphics[width = 1\textwidth]{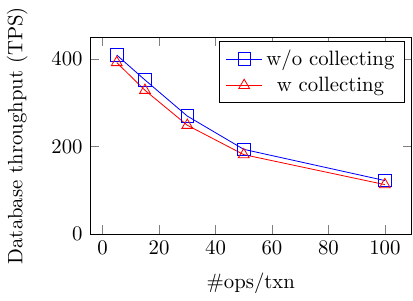}
		\caption{Database throughputs with and without collecting history.}
		\label{fig:exp-online-throughput-ops}
	\end{minipage}
	\hfill
	\begin{minipage}{0.23\textwidth}
		\centering
		\includegraphics[width = 1\textwidth]{figs/exp-online-gc}
		\caption{Memory usage of \onlinetool{} over time.}
		\label{fig:exp-online-gc}
	\end{minipage}
\end{figure}
