# Supplementary material for: Online Timestamp-based Transactional Isolation Checking of Database Systems (Extended Version)
Source: arXiv:2504.01477 source file (2025-04-02)
Supplement: Supplementary file 35 [file exp-online-tps-cobra.tex]

% exp-online-tps-cobra.tex

\begin{figure}[t]
	\centering
	% \includegraphics[width = 0.30\textwidth]{figs/exp-online-tps-cobra.pdf}
	% \caption{Throughput of \onlinetool{} and Cobra over time.}
	% \label{fig:online-tps-cobra}
        \begin{subfigure}{0.235\textwidth}
		\centering
		\includegraphics[width = \textwidth] {figs/exp-online-tps-cobra.pdf}
		\caption{SER checking (Default)}
		\label{fig:online-tps-cobra}
	\end{subfigure}
        \begin{subfigure}{0.235\textwidth}
		\centering
		\includegraphics[width = \textwidth] {figs/exp-online-tps-aionsi.pdf}
		\caption{SI checking (Default)}
		\label{fig:online-tps-si-check}
	\end{subfigure}
        \begin{subfigure}{0.235\textwidth}
		\centering
		\includegraphics[width = \textwidth] {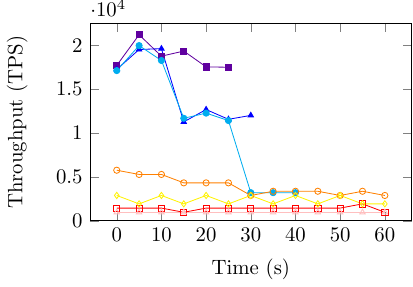}
		% \caption{\revise{SER checking (RUBiS)}}
            \caption{SER checking (RUBiS)}
		\label{fig:online-tps-rubis-ser}
	\end{subfigure}
 %        \begin{subfigure}{0.235\textwidth}
	% 	\centering
	% 	\includegraphics[width = \textwidth] {figs/exp-online-tps-rubis-si.pdf}
	% 	\caption{SI checking (RUBiS)}
	% 	\label{fig:online-tps-rubis-si}
	% \end{subfigure}
        \begin{subfigure}{0.235\textwidth}
		\centering
		\includegraphics[width = \textwidth] {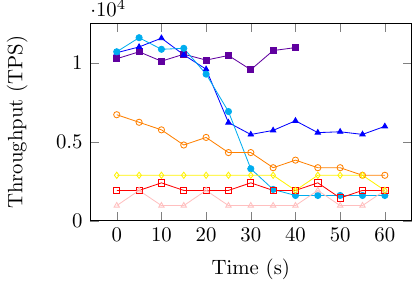}
		% \caption{\revise{SER checking (Twitter)}}
            \caption{SER checking (Twitter)}
		\label{fig:online-tps-twitter-ser}
	\end{subfigure}
 %        \begin{subfigure}{0.235\textwidth}
	% 	\centering
	% 	\includegraphics[width = \textwidth] {figs/exp-online-tps-twitter-si.pdf}
	% 	\caption{SI checking (Twitter)}
	% 	\label{fig:online-tps-twitter-si}
	% \end{subfigure}
    \caption{Throughput of online checking over time.}
    \label{fig:online-tps-throughput}
\end{figure}
