# Supplementary material for: Online Timestamp-based Transactional Isolation Checking of Database Systems (Extended Version)
Source: arXiv:2504.01477 source file (2025-04-02)
Supplement: Supplementary file 36 [file exp-online-tps.tex]

% exp-other-tools-elle.tex

\begin{figure}[t]
	\begin{subfigure}{0.235\textwidth}
		\centering
		\includegraphics[width = \textwidth] {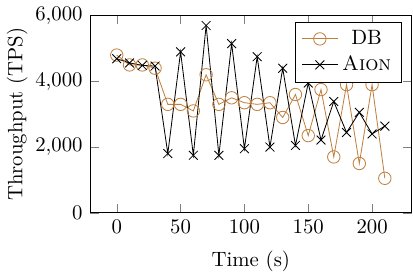}
		\caption{In seconds}
		\label{fig:exp-online-tps-sec}
	\end{subfigure}
	\begin{subfigure}{0.235\textwidth}
		\centering
		\includegraphics[width = \textwidth] {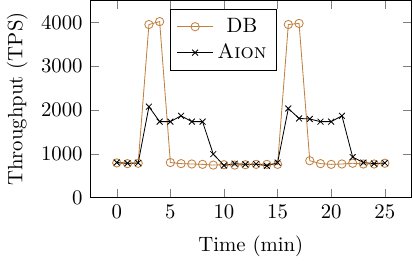}
		\caption{In minutes}
		\label{fig:exp-online-tps-min}
	\end{subfigure}
	\caption{Throughputs of both database and \onlinetool.}
	\label{fig:exp-online-tps}
\end{figure}
