# Supplementary material for: Online Timestamp-based Transactional Isolation Checking of Database Systems (Extended Version)
Source: arXiv:2504.01477 source file (2025-04-02)
Supplement: Supplementary file 40 [file latency-stat.tex]

% latency-stat.tex

\begin{figure}[t]
	\centering
	\includegraphics[width = 0.25\textwidth]{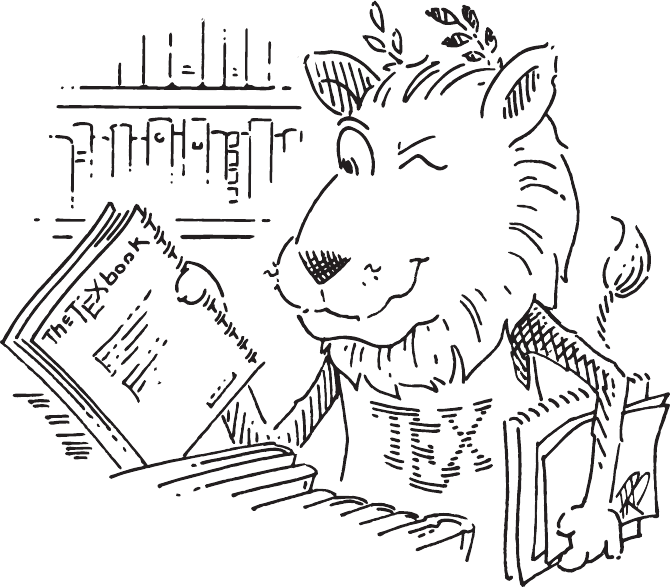}
	\caption{Statistics of network delays between the checker
	  and the database instances.
		\red{one figure has three boxplots of pgfplots;
		each boxplot: min, max, median, 25\%, 75\%, etc of the delays
		between the checker and one database instance.
		show the numbers for the medians}}
	\label{fig:latency-stat}
\end{figure}
