# Supplementary material for: Online Timestamp-based Transactional Isolation Checking of Database Systems (Extended Version)
Source: arXiv:2504.01477 source file (2025-04-02)
Supplement: Supplementary file 41 [file latency-throughput.tex]

% latency-throughtput.tex

\begin{figure}[t]
	\centering
	\begin{subfigure}[b]{0.20\textwidth}
    \centering
    \includegraphics[width = \textwidth]{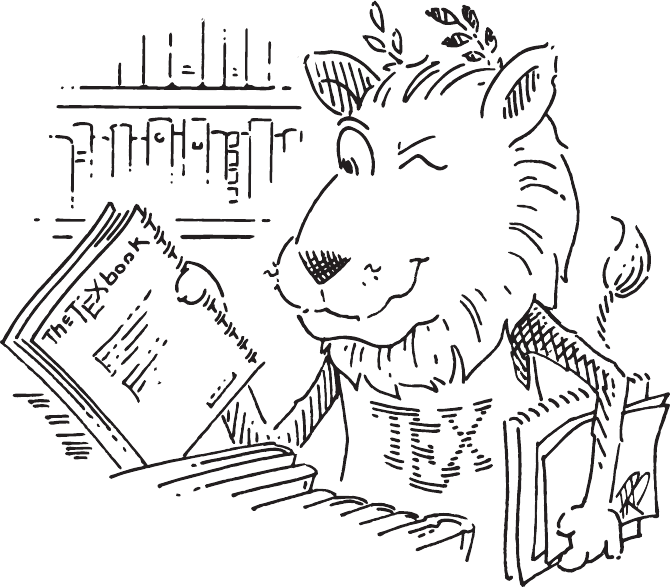}
    \caption{YugabyteDB}
    \label{fig:latency-throughput-yugabytedb}
  \end{subfigure}
	\hfill
	\begin{subfigure}[b]{0.20\textwidth}
    \centering
    \includegraphics[width = \textwidth]{figs/ctanlion}
    \caption{TiDB}
    \label{fig:latency-throughput-tidb}
  \end{subfigure}
	\hfill
	\begin{subfigure}[b]{0.20\textwidth}
    \centering
    \includegraphics[width = \textwidth]{figs/ctanlion}
    \caption{MongoDB}
    \label{fig:latency-throughput-mongodb}
  \end{subfigure}
	\hfill
	\begin{subfigure}[b]{0.20\textwidth}
    \centering
    \includegraphics[width = \textwidth]{figs/ctanlion}
    \caption{Dgraph}
    \label{fig:latency-throughput-dgraph}
  \end{subfigure}
	\caption{\red{(see Figure~12 of Cobra; four subfigs for four databases;
		each subfig has four lines: Cobra, normal, \onlinetool, \onlinetool{} with GC)}
	  Latency and throughput of \onlinetool{} for TPC-C benchmark.}
	\label{fig:latency-throughput}
\end{figure}
