# Supplementary material for: Online Timestamp-based Transactional Isolation Checking of Database Systems (Extended Version)
Source: arXiv:2504.01477 source file (2025-04-02)
Supplement: Supplementary file 46 [file stability.tex]

% stabliity.tex

\begin{figure}[t]
	\centering
	\begin{subfigure}[b]{0.15\textwidth}
    \centering
    \includegraphics[width = \textwidth]{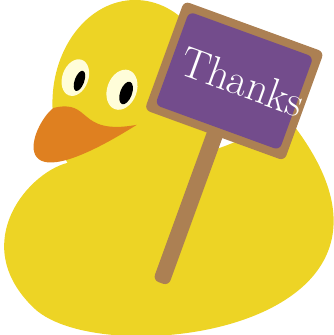}
    \caption{$\sim N(50, 0)$.}
    \label{fig:stability-50ms}
  \end{subfigure}
	\hfill
	\begin{subfigure}[b]{0.15\textwidth}
    \centering
    \includegraphics[width = \textwidth]{figs/thx-duck}
    \caption{$\sim N(100, 0)$.}
    \label{fig:stability-100ms}
  \end{subfigure}
	\hfill
	\begin{subfigure}[b]{0.15\textwidth}
    \centering
    \includegraphics[width = \textwidth]{figs/thx-duck}
    \caption{$\sim N(200, 0)$.}
    \label{fig:stability-200ms}
  \end{subfigure}
	\caption{Stability of \onlinetool{} in terms of
	  flip-flops between false positives and false negatives
		on \extaxiom. \red{three subfigs for three random delays;
		each subfig is a histogram (pgfplots)}}
	\label{fig:stability}
\end{figure}
