# Supplementary material for: Online Timestamp-based Transactional Isolation Checking of Database Systems (Extended Version)
Source: arXiv:2504.01477 source file (2025-04-02)
Supplement: Supplementary file 50 [file newcommands.tex]

% newcommands.tex

% math

% table

% font
 % bf + it: \emph{\textbf{#1}}

%%%%%%%%%%%%%%% system models %%%%%%%%%%%%%%%

%%%%%%%%%%%%%%% system models %%%%%%%%%%%%%%%

%%%%%%%%%%%%%%% axioms %%%%%%%%%%%%%%%

%%%%%%%%%%%%%%% axioms %%%%%%%%%%%%%%%

%%%%%%%%%%%%%%% checking %%%%%%%%%%%%%%%

%%%%%%%%%%%%%%% checking %%%%%%%%%%%%%%%

% colors

\colorlet{lightteal}{teal!60}

% math

 % for powerset
 % or using <>?
 % or using (#1)?

%%%%%%%%%%%%%%% rs-tx %%%%%%%%%%%%%%%

%%%%%%%%%%%%%%% rs-tx %%%%%%%%%%%%%%%

%%%%%%%%%%%%%%% evaluation %%%%%%%%%%%%%%%

%%%%%%%%%%%%%%% evaluation  %%%%%%%%%%%%%%%

% style

 % \leftturn
