# Supplementary material for: Online Timestamp-based Transactional Isolation Checking of Database Systems (Extended Version)
Source: arXiv:2504.01477 source file (2025-04-02)
Supplement: Supplementary file 52 [file ack.tex]

% ack.tex

\begin{acks}
	This work is supported by
\end{acks}
