# Supplementary material for: Online Timestamp-based Transactional Isolation Checking of Database Systems (Extended Version)
Source: arXiv:2504.01477 source file (2025-04-02)
Supplement: Supplementary file 53 [file complexity.tex]

% complexity.tex

%%%%%%%%%%%%%%%%%%%%%%%%%%%%%%
\subsection{Time and Space Complexity}
\label{ss:complexity}

%%%%%%%%%%%%%%%%%%%%%%%%%%%%%%
