# Supplementary material for: Online Timestamp-based Transactional Isolation Checking of Database Systems (Extended Version)
Source: arXiv:2504.01477 source file (2025-04-02)
Supplement: Supplementary file 73 [file size.tex]

% size.tex

\begin{table}[]
  \centering
  \caption{Log (with and without timestamps) size and history size per 1k transactions.
	  The notation $x/y/z$ shows the log size with timestamps,
		the log size without timestamps,
		and the history size, respectively.
		All the numbers are in KB.}
  \label{table:size}
  \resizebox{\columnwidth}{!}{%
  \begin{tabular}{|c|c|c|c|c|}
    \hline
              & YugabyteDB & TiDB & MongoDB & Dgraph \\ \hline
    TPC-C     & $x/y/z$           &      &         &        \\ \hline
    C-RUBiS   &            &      &         &        \\ \hline
    C-Twitter &            &      &         &        \\ \hline
  \end{tabular}%
  }
\end{table}
