# Supplementary material for: Online Timestamp-based Transactional Isolation Checking of Database Systems (Extended Version)
Source: arXiv:2504.01477 source file (2025-04-02)
Supplement: Supplementary file 74 [file ts-cost.tex]

% ts-cost.tex

\begin{table}[]
	\centering
	\caption{Lightweight methods of extracting timestamps from
	  the four representative databases.}
	\label{table:ts-cost}
  
	\resizebox{\columnwidth}{!}{%
		\begin{tabular}{|c|ccc|cc|}
		\hline
		\multirow{2}{*}{DBMS}       & \multicolumn{3}{c|}{Cost (source code modification)}
																& \multicolumn{2}{c|}{GitHub Issues}  \\ \cline{2-6}
																& \multicolumn{1}{c|}{Source}
																& \multicolumn{1}{c|}{Changes}
																& Description
																& \multicolumn{1}{c|}{Links}
																& Status \\ \hline
		\multirow{2}{*}{MongoDB}    & \multicolumn{1}{c|}{}
																& \multicolumn{1}{c|}{}
																&
																& \multicolumn{1}{c|}{}
																&        \\ \cline{2-6}
																& \multicolumn{1}{c|}{}
																& \multicolumn{1}{c|}{}
																&
																& \multicolumn{1}{c|}{}
																&        \\ \hline
		\multirow{2}{*}{YugabyteDB} & \multicolumn{1}{c|}{}
																& \multicolumn{1}{c|}{}
																&
																& \multicolumn{1}{c|}{}
																&        \\ \cline{2-6}
																& \multicolumn{1}{c|}{}
																& \multicolumn{1}{c|}{}
																&
																& \multicolumn{1}{c|}{}
																&        \\ \hline
		\multirow{2}{*}{TiDB}       & \multicolumn{1}{c|}{}
																& \multicolumn{1}{c|}{}
																&
																& \multicolumn{1}{c|}{}
																&
																\\ \cline{2-6}
																& \multicolumn{1}{c|}{}
																& \multicolumn{1}{c|}{}
																&
																& \multicolumn{1}{c|}{}
																&        \\ \hline
		\multirow{1}{*}{Dgraph}     & \multicolumn{1}{c|}{\textsf{txn.py} in \textsf{pydgraph}}
																& \multicolumn{1}{c|}{c1}
																& add return value to \textsf{commit}
																& \multicolumn{1}{c|}{{\cite{pydgraph-txn}}}
																& {PR Merged~\cite{pydgraph-pr}}
																% \\ \cline{2-6}
																% & \multicolumn{1}{c|}{}
																% & \multicolumn{1}{c|}{}
																% &
																% & \multicolumn{1}{c|}{}
																% &        \\ \hline
																\\ \hline
		\end{tabular}%
	}
\end{table}
