# Supplementary material for: Online Timestamp-based Transactional Isolation Checking of Database Systems (Extended Version)
Source: arXiv:2504.01477 source file (2025-04-02)
Supplement: Supplementary file 75 [file workload.tex]

% workload.tex

\begin{table}[t]
  \centering
  \caption{Parameters of default workload.}
  \label{table:workload-parameters}
  
  \resizebox{\columnwidth}{!}{%
    \begin{tabular}{|c|c|c|}
      \hline
      \textbf{Parameters}   & \textbf{Values}  & \textbf{Default} \\ \hline
      \hline
      Number of sessions (\#sess)
          & $10$, $20$, $50$, $100$, $200$
          & $50$    \\ \hline
      Number of transactions (\#txns)
          & \incell{c}{$5$K, $100$K, $200$K, $500$K, $1, 000$K}
          & $100$K  \\ \hline
      \incell{c}{Number of operations per transaction\\(\#ops/txn)}
          & $5$, $15$, $30$, $50$, $100$
          & $15$    \\ \hline
      % \incell{c}{Ratio of read-only transactions (\%ro)}
      %     & $0\%$, $25\%$, $50\%$, $75\%$
      %     & $50\%$  \\ \hline
      \incell{c}{Ratio of read operations (\%reads)}
          & $10\%$, $30\%$, $50\%$, $70\%$, $90\%$
          & $50\%$  \\ \hline
      Number of keys (\#keys)                      & $200$, $500$, $1000$, $2000$, $5000$   & $1000$  \\ \hline
      Distribution of key access (dist)          & Uniform, Zipfian, Hotspot              & Zipfian \\ \hline
    \end{tabular}%
  }
\end{table}
