# Supplementary material for: Online Timestamp-based Transactional Isolation Checking of Database Systems (Extended Version)
Source: arXiv:2504.01477 source file (2025-04-02)
Supplement: Supplementary file 76 [file packages.tex]

% packages.tex

\usepackage{amsmath,amssymb,amsfonts}
\usepackage{amsthm}
\usepackage{wasysym}
% for two-column algorithms
% see https://tex.stackexchange.com/a/159431.
\usepackage{varwidth}
\usepackage{algorithm}
\usepackage{url}
% \usepackage{algorithmic}
\usepackage[noend]{algpseudocode}
% \algrenewcommand{\algorithmiccomment}[1]{\hfill {\color{gray} #1}}
% \usepackage{paralist}
\usepackage{array}

% \usepackage{wasysym}
\usepackage[clock]{ifsym}

\usepackage{fontawesome}

\usepackage{multirow}

\usepackage{pifont}

\usepackage{caption}
\usepackage{subcaption}

\usepackage{graphicx}
\usepackage[export]{adjustbox}

\usepackage{balance}

% \usepackage{amsmath,amssymb,amsfonts}
\usepackage{xcolor}

\usepackage{enumitem}

% \usepackage{ulem}

% below does not work; do not know why
% \usepackage{xcolor}
% \usepackage{hyperref}
% \hypersetup{
%   colorlinks,
%   citecolor=violet,
%   linkcolor=red,
%   urlcolor=blue}
