# Supplementary material for: Online Timestamp-based Transactional Isolation Checking of Database Systems (Extended Version)
Source: arXiv:2504.01477 source file (2025-04-02)
Supplement: Supplementary file 77 [file cover_letter.tex]

\newcommand{\comments}[2]{\noindent{\textbf{Comment #1}}: {#2}}
\newcommand{\response}[2]{\vspace{2mm}\noindent\textbf{Response #1}: {#2} \vspace{0.5mm}}
\newcommand{\revhighlight}[1]{\emph{\textbf{\uuline{#1}}}}
\pagestyle{empty}
\thispagestyle{empty}

% \newcommand{\question}[1]{}
\newcommand{\question}[1]{{\textcolor{blue}{(#1)}}}

\onecolumn

\centerline{\textbf{\Large Responses to Reviewers' Comments}}
\vspace{1mm}

\begin{multicols}{2}

\setcounter{page}{1}

\noindent We would like to thank the reviewers and meta reviewer for their constructive comments.
We have addressed all the comments in the revised paper.
We highlight the major revisions in {\color{blue} blue}.

\section*{Summary of Changes}
\begin{itemize}
    \item \textbf{Evaluation (R1.O1, R4.\{O2,O3,O4,O5,O6\}) :}
    We have substantially improved the experiments in Section \ref{ss:throughput} according to the reviewers' constructive comments. 
    In particular, we have conducted new experiments
    on two more datasets/workloads and on non-conforming histories.
    We also improved our setup, descriptions, and discussions of evaluations.
    \item \textbf{Discussion (R3.\{O3,D2\}, R4.O1) :}
    Our method applies to general SQL features and MVCC databases,
    as long as we can infer the versions/snapshots order of transactions
    in a history.
    We have discussed the limitations on SQL features
    and databases supported in Section \ref{section:conclusion}. 
    \item \textbf{Clarification (R1.D1, R3.\{O1,O2,D1\}, R4.O7) :} 
    We discuss the correctness of the online checking algorithm
    \onlinetool{} with respect to the out-of-order arrival of transactions.
    We also describe our timeout mechanism in Section \ref{ss:workflow} and transaction abort handling in Section \ref{ss:generating-workloads} in the revised manuscript. 
\end{itemize}

\section*{Response to Meta-Reviewer}

We have addressed all the required changes accordingly. 
Please refer to our responses to Reviewers R1, R3, and R4 below for details.

% \newcolumn
\section{Response to Reviewer \#1}
\begin{framed}
\textit{O1: The benchmark utilized, although showing varied parameters, is generic and may not reflect industry-strenght workloads. Specially considering the work proposes a serializability checker, it would be important to include a golden-standard OLTP benchmark, such as TPC-C. Compared to viper, which contains TPC-C, RUBiS, Twitter workloads, this work lags behind in the benchmark settings.}
\end{framed}
\response{O1}{
We sincerely appreciate your insightful feedback on this crucial issue. To enhance the practicality of our research, in this revision, we've incorporated the RUBiS and Twitter workloads as suggested. We integrated these workloads into our experiments to comprehensively evaluate our proposed online checker, \onlinetool{}. 

Figure~\ref{fig:online-tps-rubis-ser} and Figure~\ref{fig:online-tps-twitter-ser} show similar results for different datasets. \onlinetool{} still outperforms Cobra in checking throughput against new datasets.
Notably, \onlinetool's throughput decreases on the Twitter dataset compared to RUBiS,
due to the increasing number of keys,
requiring high computation and storage
to maintain the data structure $\frontierts$.
Cobra's performance depends on transaction dependencies,
influenced by key distribution, read-write ratios, and the number of operations per transaction,
rather than the number of keys.

The detailed results and analysis of the evaluation are presented in Section \ref{ss:throughput} of the revised paper.
The experimental results for \onlinetool{}-SI are similar,
we move them to the appendix of technical report \cite{aion_and_chronos}.

For the TPC-C benchmark,
we have evaluated \tool{} instead of \onlinetool{}
due to TPC-C's extensive use of composite primary keys,
which results in a large key space.
\onlinetool{} requires maintaining a frontier for each timestamp,
i.e., $\frontierts$, demanding significant computational and memory resources,
as seen in the Twitter vs. RUBiS comparison.
In contrast, \tool{} maintains a single global frontier,
making it well-suited for handling TPC-C.

While \tool{} outperforms Cobra in Twitter and RUBiS
(where Cobra encounters out-of-memory errors with a large number of transactions, e.g., 500K),
we aim to enhance \onlinetool’s algorithm
and implementation to address the large key space issue.
Cobra, though unaffected by this issue,
does not qualify as a true online checker,
as it modifies client workloads
(e.g., inserting fence transactions \cite{Cobra:OSDI2020} and batching offline histories) and halts upon detecting a violation (see R4.O6).

%is absent in our work, as the TPC-C benchmark is robust \cite{RobustnessSI:CAV2019,DBLP:journals/pvldb/VandevoortK0N21:robustness} under the SI level, meaning TPC-C history is Serializable when running it under SI level. Since our work focuses on both the SER and SI scenarios, the TPC-C benchmark does not effectively test the capabilities of our checker and SOTA method in the SER context. Therefore, we decided not to include it in this round of experiments. However, we recognize the importance of the TPC-C benchmark and plan to explore its applicability in future research, potentially using it to better evaluating the SI scenario.
}

% \newcolumn
\begin{framed}
\textit{D1: In TiDB, where are the transaction timestamps extracted from?}
\end{framed}

\response{D1}{
To obtain the timestamps of each transaction in TiDB, we modify its source code for CDC (Change Data Capture) to expose them by adding just logging statements. The source code can be found at \cite{tidb_ts_get}. We have added this into Section \ref{ss:extracting-timestamps} of the revised manuscript.
}

% \newcolumn
\section{Response to Reviewer \#3}

\begin{framed}
\textit{O1: The paper lacks a formal proof of correctness for the online AION algorithm. This omission raises questions about the algorithm's theoretical soundness.}
\end{framed}

\response{O1}{
Thank you for your suggestion. The \onlinetool{} algorithm follows a ``simulate-and-check'' approach, and its correctness is straightforward when all transactions are processed in ascending order based on their start/commit timestamps, ensuring no re-checking is required. However, when out-of-order transactions necessitate re-checking, it is crucial to determine which transactions should be re-checked against which axioms.

Suppose that a transaction $T$ arrives out of order. We divide the set of previously processed transactions into three categories and, for each category (fixing a representative transaction $T'$), identify the set of axioms that should be re-checked. Clearly, the \intaxiom{} axiom for $T$' is not influenced by $T$ and thus does not need to be re-checked.
\begin{itemize}
    \item $T'$ commits before $T$ starts: $T'$ is not influenced by $T$, so no axioms need to be re-checked.
    \item $T'$ commits after $T$ starts but starts before T commits: Since a transaction only considers transactions that committed before it as visible, the \extaxiom{} axiom for $T'$ does not need to be re-checked. However, since $T'$ overlaps with $T$, we must re-check the \noconflictaxiom{} axiom.
    \item $T$' starts after $T$ commits: The \extaxiom{} axiom needs to be re-checked, but the \noconflictaxiom{} axiom does not.
\end{itemize}

We have added the insight in Section \ref{ss:aion} and the formal argument to the appendix of the technical report \cite{aion_and_chronos} due to space constraints. 
}

\begin{framed}
\textit{O2: The timeout mechanism is underexplained. The criteria for setting timeout values and its implications for correctness (e.g., missed transactions causing false violations) should be clarified.}
\end{framed}

\response{O2}{
The timeout mechanism sets a deadline for checking and re-checking the \extaxiom{} axiom for each transaction. Within this period, \onlinetool{}  does not report the \extaxiom{} violation as it is subject to change due to asynchrony. Once the timeout expires, the \extaxiom{} checking result is considered final and is reported to clients.

To ensure the correctness of the final result, the timeout value should be set so that no more transactions arrive out of order after the timeout expires. This is determined based on system parameters such as network latency and clock skew. In our experiments, we conservatively set 5 seconds. 
We have added this clarification in Section \ref{ss:workflow}.
}

\begin{framed}
\textit{O3: More discussion is needed on scenarios where databases do not expose timestamp information or fail to meet timestamp property assumptions.}
\end{framed}

\response{O3}{
Our approach uses timestamps to infer the transaction execution order and/or determine the snapshot of each transaction. Therefore, it does not directly work for database systems which implement SI/SER using mechanisms distinct from the timestamp-based methods. However, our approach still can be generalized to handle more database systems.

For example, PostgreSQL associates each transaction with a unique ID and guarantees that concurrent transactions are committed in the increasing order of their IDs in its SSI implementation \cite{DBLP:journals/pvldb/PortsG12_postgresql_SSI_implementation}. Therefore, we can treat such IDs as commit timestamps in our approach, and these IDs can be easily extracted from the log. For example, Emme \cite{Clark:EuroSys2024} leverages PostgreSQL’s logical streaming replication and the Debezium's CDC tool to recover the version order, which is defined as the commit order of transactions. We will explore these two methods in the future work.
In their SI implemenations, databases like SQL Server \cite{SQLServer}, PostgreSQL \cite{PostgreSQL}, and WiredTiger \cite{WiredTiger-Transaction} rely on the visibility rules to compute a transaction’s snapshot. They associate each transaction with a unique ID, but the transaction IDs, such as those used in WiredTiger, may not directly correlate with the timestamps employed in the database systems considered in this paper. We will explore how to obtain the snapshots in a lightweight way in these databases in the future work.
We have added a discussion in Section \ref{section:conclusion} of the revised manuscript.
}

\begin{framed}
\textit{D1: The handling of transaction aborts in an online environment is not discussed. In an offline environment they can be filtered out, so this omission could leave gaps in the implementation for online processing.}
\end{framed}

\response{D1}{
In theory, we follow the convention that all transactions in history are assumed to be committed \cite{Framework:CONCUR2015}. That is, the specifications do not constrain values read inside aborted transactions.

In implementation, we ignore aborted transactions in the logs.  Specifically, we collect only committed transactions and send them to both the offline and online checkers. This is justified by the common assumption that an underlying recovery mechanism will rollback aborted transactions \cite{AllocatingIsolation:PODS2005,DBLP:conf/pods/VandevoortKN23:PODS2023,Robustness:CONCUR2016}.

As developed in the textbook \cite{DBLP:books/mk/WeikumV2002:book} (Chapter 11), it is quite non-trivial to formalize the notion of transaction recovery: the expanded history and the condition of (conflict) serializability should take into account the undo operations. In this work, we do not test the recovery mechanism and simply assume it works correctly.
We have added a description in Section \ref{ss:generating-workloads}.
}

\begin{framed}
\textit{D2: Rollback to savepoints, a feature in many databases, is not addressed. Its inclusion would enhance practical applicability.}
\end{framed}

\response{D2}{
The intra-transaction savepoints are useful for partial rollbacks which can be supported by the underlying recovery algorithm. As discussed in our response to R3.D1, we do not test the recovery mechanism and simply assume it works correctly.
That said, it would be valuable to extend our work to support both intra-transaction savepoints and aborted transactions. We have added a short discussion in Section \ref{section:conclusion} of the revised manuscript and will explore these issues in future work.
}

\clearpage

% \newcolumn
\section{Response to Reviewer \#4}
\begin{framed}
    \textit{O1: The approach cannot be applied to complex SQL queries as described because it relies on knowing all keys involved in reads and writes (no general predicates). This is mentioned as future work but does limit the usefulness of the checkers.}
\end{framed}



\response{O1}{Our approach can be easily generalized to support SQL predicates, as long as we can infer the commit order and/or snapshots of transactions from their start and commit timestamps generated by the database system. Specifically, our approach simulates the execution of transactions in ascending commit order, and check corresponding axioms on the fly. The key to support predicates is to determine the version set (defined in \cite{Adya:PhDThesis1999}) of each predicate-based operation of a transaction, according to the snapshot taken by the transaction. Based on this idea, \cite{Clark:EuroSys2024} provides an offline SER checking algorithm supporting predicates, which we will generalize to the online setting. We have added more discussions in Section \ref{section:conclusion} of the revised manuscript.
}

\begin{framed}
\textit{O2: The workload used for the evaluation is synthetic and seems quite simple (YCSB-like except with multiple operations per transaction). I couldn't find the (Python?) source code for the workload from a quick look through the anonymous github repo or some of the figure artifacts, only files with pre-generated traces. A more thorough description of the workload than table 1, or better yet, an evaluation with an existing workload, would strengthen the paper.}
\end{framed}

\response{O2}{
Thank you for your valuable suggestions. In this revision, we have conducted additional experiments using industry benchmarks including Twitter and RUBiS.
For details, please refer to our response to R1-O1 and revision in Section \ref{ss:throughput} of the revised paper. 

We have added more detailed descriptions of the workloads, including their generation and the test scenarios in Sections \ref{sss:perf-setup} and \ref{ss:online-setup}.
Additionally, we have updated our repo \cite{aion_and_chronos}
with all source code, including that for generating the workloads.}

\begin{framed}
\textit{O3: Figure 15 suggests that the database throughput is only 400 TPS even with small \#ops / txn. Is this correct and if so, am I understanding that the throughput of Aion shown in Figure 12 50x faster? What I'm interested in is whether there is a point where Aion cannot keep up with the throughput of the database or runs out of memory with a steady state workload, but I can figure that out from the evaluation.}
\end{framed}

\response{O3}{
The throughput values in Figure \ref{fig:online-throughput} and Figure \ref{fig:online-tps-throughput} are obtained under different settings and should not be directly compared. The experiment in Figure \ref{fig:online-throughput} evaluates the impact of history collection on database throughput, showing that collecting and transmitting the history results in a roughly 5\% decrease in database throughput. This experiment was conducted on a lower-spec machine running a three-node Dgraph cluster in real-time, leading to lower database throughput.
In contrast, the experiment in Figure \ref{fig:online-tps-throughput} measures \onlinetool{}’s peak throughput in a simulated scenario, where an offline-collected history is sent in batches to the \onlinetool{} checker. This setup evaluates \onlinetool{}’s maximum capacity under extreme database throughput conditions.
From Figure \ref{fig:online-tps-throughput}, we observe that during steady-state scenario, where \onlinetool{} performs both checking and garbage collection, it maintains a throughput of approximately 12K TPS. This represents the threshold at which \onlinetool{} can keep up with database throughput.
We have clarified this discussion in Section \ref{ss:online-setup} of the revised manuscript. Additionally, we have conducted further experiments using existing benchmarks in this revision. For details, please refer to our response to R1.O1.
}

\begin{framed}
\textit{O4: The performance of both Chronos and Aion are highly dependent on GC (Figs 9, 10, 12). This seems like a challenge for online use in particular. The evaluation only considers 100K transactions but many real-world DBMSes can process 100K txn/s. Fig 16 suggests it might take 310 seconds to check these. The paper should clarify the conditions for Aion to run online checking continuously.}
\end{framed}

\response{O4}{
Thank you for your feedback. We acknowledge that GC impacts the performance of both \tool{} and \onlinetool{}, particularly in online scenarios, and timely GC is necessary to prevent memory constraints and a lower GC frequency improves performance. In the offline setting, the performance bottleneck of \tool{} does not lie in GC, but in loading and parsing the history file. As shown in Figure \ref{fig:memory-default}, memory usage initially increases gradually, but after manually triggering a JVM GC at the end of the loading phase, there is a sudden and significant drop. During the checking phase, memory usage fluctuates based on GC frequency, but even without any GC (indicated by the blue line), memory usage at the end of checking is still much lower than at the end of loading. This indicates that the peak memory usage occurs at the end of loading, highlighting that the bottleneck lies in loading files into memory rather than in GC.

Figure \ref{fig:exp-online-throughput-memory} shows that it takes \onlinetool{} approximately 310 seconds to check 100K transactions in the online setting, including both the database execution time and the checking time. In this experiment, the performance bottleneck lies in the database throughput. Because, as shown in Figure \ref{fig:online-tps-si-check}, \onlinetool{} can check 500K transactions in approximately 30 seconds, when the arrival rate of transactions exceeding 25K TPS. 
\onlinetool{}'s checking speed (on average 12K TPS) meets the requirements of large-scale businesses. For example, Visa processed 639 million transactions per day in 2024, averaging less than 8K TPS \cite{visa-fact-sheet}. We acknowledge that some databases can achieve 100K TPS or higher during peak periods. While \onlinetool{} may not always keep up with peak TPS, it can exceed TPS during off-peak periods and eventually catch up. If the sustained TPS consistently exceeds \onlinetool{}’s checking speed, we recommend scaling resources or switching to an offline algorithm for efficient verification. We have clarified this in Section \ref{ss:throughput} of the revised manuscript.
%Additionally, we have conducted further experiments using existing benchmarks in this revision. For details, please refer to our response to R1.O1.
}

\begin{framed}
\textit{O5: There are many experiments described, and it is not always clear (a) which DBMS is used to generate histories, and (b) whether the parameters for each experiment build on the previous one or are independent. This applies particularly to Figure 12-16: please make sure each can be understood fully by reading the caption and the associated text description.}
\end{framed}

\response{O5}{
Thank you for your feedback. 
(a) To improve clarity, we have explicitly stated the DBMS used for each experiment and clarified the dependencies between experiments. 

(a) Specifically, for the Twitter and RUBiS datasets,
we collect SER- and SI-consistent histories from Dgraph (v20.03.1). For the default dataset, we use SI histories collected from Dgraph (v20.03.1) operating on a key-value store.
However, as Dgraph lacks support for list data types,
we use SI histories collected from TiDB (v7.1.0) for comparing \tool{} with ElleList. For SER checking, we collect histories from YugabyteDB (v2.20.7.1). We revise it in Section \ref{sss:perf-setup}. 

(b) In our test scenarios, the database throughput is lower than the checking speed (as shown in Figure 13-16).
To evaluate \onlinetool{}'s throughput limits,
we pre-collected logs and then fed historical data
exceeding the checkers' throughput (see Figure 12).
We revise it in Section \ref{ss:online-setup}. 

The overall TPS (Transactions Per Second) is relatively low
due to three factors:
1) subpar hardware;
2) slow throughput of the distributed database;
and 3) low performance of the disk-based and graph databases when handling relational tables.
}

\begin{framed}
\textit{O6: All the testing described is to measure performance for checking conforming histories. It would strengthen the paper to describe testing with histories containing anomalies ensuring that all violations are detected.}
\end{framed}

\response{O6}{Thank you for your suggestion.
In this revision, we have conducted additional experiments using existing benchmarks;
for details, please refer to our response to R1.O1.

We also used a history with 500K transactions generated under the SI level to test \onlinetool{}-SER.
The result shows that \onlinetool{} efficiently detects all 11839 violations with a checking speed comparable to that on violation-free histories, while Cobra terminates upon detecting the first violation.
We have validated the number of violations by \tool{}-SER.

We have added the non-conforming conclusion in Section \ref{ss:throughput} in the revised manuscript and, due to space constraints, similar experimental figures to the technical report \cite{aion_and_chronos}}

\begin{framed}
\textit{O7: The Aion-SER implementation assumes that transactions are "executed sequentially in the commit timestamp order". In this case, I don't understand why any checking is needed: can you please explain? Further, SER histories were collected from YugabyteDB, which uses locking (S2PL) to enforce SER. Would the approach work with PostgreSQL, which uses Serializable Snapshot Isolation?}
\end{framed}

\response{O7}{
Sorry for the confusion. In Section \ref{ss:online-setup} of the revised manuscript, we have rephrased this sentence as follows: ``The \onlinetool{}-SER algorithm checks whether all transactions appear to execute sequentially in commit timestamp order.'' 
For the feasibility and generalizability of our approach on PostgreSQL, please refer to our response to R3.O3.
}

\begin{framed}
\textit{D1 Writing issue: The paper follows ICDE inclusive writing guidelines as far as I can see. Readability could be enhanced by making some figures larger but this may require omitting some figures to stay within the page count.}
\end{framed}

\response{D1}{Due to space constraints,
we guarantee that all figures are lossless
and can be enlarged for better readability.
We have also added all high-quality figures to the repo \cite{aion_and_chronos}.}

\begin{framed}
\textit{D2 Availability: The github repo contains the main tool, which looks good to me. The per-figure artifacts seem to contain pre-generated traces that can be processed. I was hoping to see the system working end-to-end (a workload driving a DBMS with traces captured and fed to Aion online). Maybe I missed it?}
\end{framed}

\response{D2}{We thank all the reviewers for their efforts in evaluating our artifact.
We have added more descriptions regarding the generation and processing of workloads, including scripts and source code,
available at \cite{aion_and_chronos}.}

\vspace{2mm}
Due to \textbf{space constraints}, we have streamlined the evaluation text of \tool{} and the related work while ensuring that all key information and content remain intact. Although we have addressed all reviewer comments, not all content has been included in the main text; additional details can be found in the technical report \cite{aion_and_chronos}.
We welcome any further suggestions from the reviewers.

\end{multicols}

\twocolumn

% \clearpage
